# Supplementary material for: Spin Reorientation Driven Renormalization of Spin-Phonon Coupling in Fe$_4$GeTe$_2$
Source: arXiv:2512.18544 ancillary file (2025-12-21)
Supplement: Supplementary file 1 [file Supporting_Information.pdf]

# Supporting Information

## Spin Reorientation Driven Renormalization of Spin–Phonon Coupling in $Fe_4GeTe_2$

Riju Pal[1*], Md. Nur Hasan[2], Chumki Nayak[3], Mrinal Deka[4], Nastaran Salehi[2], Manuel Pereiro[2], Suchanda Mondal[5], Abhishek Misra[4], Achintya Singha[3], Prabhat Mandal[1*], Debjani Karmakar[2,6,7*], and Atindra Nath Pal[1*]

[1]*Department of Condensed Matter and Materials Physics, S. N. Bose National Centre for Basic Sciences, Block JD, Sector III, Salt Lake, Kolkata, 700106, India*
[2]*Department of Physics and Astronomy, Uppsala University, Box 516, SE-751 20 Uppsala, Sweden*
[3]*Department of Physical Sciences, Bose Institute, 93/1, Acharya Prafulla Chandra Road, Kolkata 700009, India*
[4]*Department of Physics, Indian Institute of Technology Madras, Chennai 600036, India*
[5]*Saha Institute of Nuclear Physics, HBNI, 1/AF Bidhannagar, Calcutta 700064, India*
[6]*Technical Physics Division, Bhabha Atomic Research Centre, Mumbai 400085, India*
[7]*Homi Bhabha National Institute, Mumbai, 400094, India*

Email: rijupal07@gmail.com, prabhatmandalphysics@gmail.com, karmakar.debjani@gmail.com, atin@bose.res.in

---

# Contents

**Section S1. Selection rules for Raman-active phonons**

**Section S2. $Fe_4GeTe_2$ single crystal growth, characterization, exfoliation and Raman measurement details**

**Section S3. Thickness dependent Raman measurements**

**Section S4. Laser power dependent Raman measurements**

**Section S5. Low temperature (down to 5 K) Raman measurements of 190 layered thick flake (R190) of $Fe_4GeTe_2$**

**Section S6. Additional data and analysis of R190**

**Section S7. Temperature dependent Raman measurements of 80 layered flake (R80) of $Fe_4GeTe_2$**

**Section S8 Temperature dependent Raman measurement on 8 layered thin flake (R8) of $Fe_4GeTe_2$**

**Section S9. Raman measurements of other thin $Fe_4GeTe_2$ flakes**

**Section S10. Theoretical Part**

## Section S1. Selection rules for Raman-active phonons

Single crystal $Fe_4GeTe_2$ exhibits a rhombohedral structure[1,2,3,4] with the space group $R\bar{3}m$ (No. 166), having lattice parameters a = 9.97(2) Å and α = 23.3(2)°. In the hexagonal representation, these lattice parameters are a = 4.03 Å and c = 29.08 Å. $Fe_4GeTe_2$ features trigonal crystal symmetry corresponding to the $D_{3d}$ point group. Group theory predicts that the symmetries of the Raman active modes for this structure are represented by $A_{1g}$ and $E_g$. The Raman tensors (***R***) associated with these symmetries are described[5] as follows:

$$A_{1g}: \begin{pmatrix} a & 0 & 0 \\ 0 & a & 0 \\ 0 & 0 & b \end{pmatrix}; \tag{1}$$

$$E_g: \begin{pmatrix} c & 0 & 0 \\ 0 & -c & d \\ 0 & d & 0 \end{pmatrix} \text{ and } \begin{pmatrix} 0 & -c & -d \\ -c & 0 & 0 \\ -d & 0 & 0 \end{pmatrix} \tag{2}$$

Here, the Raman active mode $A_{1g}$ is non-degenerate but the $E_g$ mode exhibits double degeneracy. The intensity of non-resonant Raman scattering for a Raman-active mode in a crystal can be determined using the Placzek approximation and is represented by the Raman tensor as follows[5]:

$$I \propto |\boldsymbol{p_i} \cdot \boldsymbol{R} \cdot \boldsymbol{p_s}|^2 \tag{3}$$

Here, the polarization vectors for incident and scattered light are represented by $\boldsymbol{p_i}$ and $\boldsymbol{p_s}$ respectively. Both $\boldsymbol{p_i}$ and $\boldsymbol{p_s}$ lie within the *xy* plane in the back-scattering configuration. Employing linearly polarized light as our basis, the polarization vectors along the *x* and *y* directions can be expressed as:

$$\boldsymbol{p_x} = (1 \quad 0 \quad 0) \tag{4}$$

$$\boldsymbol{p_y} = (0 \quad 1 \quad 0) \tag{5}$$

In the same basis, for the left ($\boldsymbol{\sigma^+}$) and right ($\boldsymbol{\sigma^-}$) circularly polarized light, the polarization vectors will be:

$$\boldsymbol{\sigma^+} = \frac{1}{\sqrt{2}}(1 \quad i \quad 0) \tag{6}$$

$$\boldsymbol{\sigma^-} = \frac{1}{\sqrt{2}}(1 \quad -i \quad 0) \tag{7}$$

### (i) For linearly parallel polarization configuration (linear ||):

Using Eq. 3, the intensities of the Raman active modes for linearly parallel polarization configuration are as follows:

$$\mathbf{I_{||}\,(A_{1g})} = \left|(1 \quad 0 \quad 0)\begin{pmatrix} a & 0 & 0 \\ 0 & a & 0 \\ 0 & 0 & b \end{pmatrix}\begin{pmatrix} 1 \\ 0 \\ 0 \end{pmatrix}\right|^2 = \left|(1 \quad 0 \quad 0)\begin{pmatrix} a \\ 0 \\ 0 \end{pmatrix}\right|^2 = |\boldsymbol{a}|^2$$

$$\mathbf{I}_{\|}\,(\mathbf{E_g}) = \left|(1\ \ 0\ \ 0)\begin{pmatrix} c & 0 & 0 \\ 0 & -c & d \\ 0 & d & 0 \end{pmatrix}\begin{pmatrix} 1 \\ 0 \\ 0 \end{pmatrix}\right|^2 + \left|(1\ \ 0\ \ 0)\begin{pmatrix} 0 & -c & -d \\ -c & 0 & 0 \\ -d & 0 & 0 \end{pmatrix}\begin{pmatrix} 1 \\ 0 \\ 0 \end{pmatrix}\right|^2$$

$$= \left|(1\ \ 0\ \ 0)\begin{pmatrix} c \\ 0 \\ 0 \end{pmatrix}\right|^2 + \left|(1\ \ 0\ \ 0)\begin{pmatrix} 0 \\ -c \\ -d \end{pmatrix}\right|^2 = |\boldsymbol{c}|^2$$

**(ii) For linearly perpendicular polarization configuration (linear ⊥):**

Similarly, using Eq. 3, the intensities of the Raman active modes for linearly perpendicular polarization configuration are as follows:

$$\mathbf{I}_{\perp}(\mathbf{A_{1g}}) = \left|(1\ \ 0\ \ 0)\begin{pmatrix} a & 0 & 0 \\ 0 & a & 0 \\ 0 & 0 & b \end{pmatrix}\begin{pmatrix} 0 \\ 1 \\ 0 \end{pmatrix}\right|^2 = \mathbf{0}$$

$$\mathbf{I}_{\perp}(\mathbf{E_g}) = \left|(1\ \ 0\ \ 0)\begin{pmatrix} c & 0 & 0 \\ 0 & -c & d \\ 0 & d & 0 \end{pmatrix}\begin{pmatrix} 0 \\ 1 \\ 0 \end{pmatrix}\right|^2 + \left|(1\ \ 0\ \ 0)\begin{pmatrix} 0 & -c & -d \\ -c & 0 & 0 \\ -d & 0 & 0 \end{pmatrix}\begin{pmatrix} 0 \\ 1 \\ 0 \end{pmatrix}\right|^2$$

$$= \left|(1\ \ 0\ \ 0)\begin{pmatrix} 0 \\ -c \\ d \end{pmatrix}\right|^2 + \left|(1\ \ 0\ \ 0)\begin{pmatrix} -c \\ 0 \\ 0 \end{pmatrix}\right|^2 = |\boldsymbol{c}|^2$$

**(iii) For co-circularly polarization configuration ($\sigma^+$ in $\sigma^+$ out):**

$$\mathbf{I}_{\sigma^+\ \text{in}\ \sigma^+\ \text{out}}(\mathbf{A_{1g}}) = \left|\frac{1}{2}\times(1\ \ i\ \ 0)\begin{pmatrix} a & 0 & 0 \\ 0 & a & 0 \\ 0 & 0 & b \end{pmatrix}\begin{pmatrix} 1 \\ -i \\ 0 \end{pmatrix}\right|^2 = |\boldsymbol{a}|^2$$

$$\mathbf{I}_{\sigma^+\ \text{in}\ \sigma^+\ \text{out}}(\mathbf{E_g}) = \left|\frac{1}{2}\times(1\ \ i\ \ 0)\begin{pmatrix} c & 0 & 0 \\ 0 & -c & d \\ 0 & d & 0 \end{pmatrix}\begin{pmatrix} 1 \\ -i \\ 0 \end{pmatrix}\right|^2 +$$

$$\left|\frac{1}{2}\times(1\ \ i\ \ 0)\begin{pmatrix} 0 & -c & -d \\ -c & 0 & 0 \\ -d & 0 & 0 \end{pmatrix}\begin{pmatrix} 1 \\ -i \\ 0 \end{pmatrix}\right|^2$$

$$= \left|\frac{1}{2}\times(1\ \ i\ \ 0)\begin{pmatrix} c \\ ic \\ -id \end{pmatrix}\right|^2 + \left|\frac{1}{2}\times(1\ \ i\ \ 0)\begin{pmatrix} ic \\ -c \\ -d \end{pmatrix}\right|^2 = \mathbf{0}$$

**(iv) For cross-circularly polarization configuration ($\sigma^+$ in $\sigma^-$ out):**

$$\mathbf{I}_{\sigma^+\ \text{in}\ \sigma^-\ \text{out}}(\mathbf{A_{1g}}) = \left|\frac{1}{2}\times(1\ \ i\ \ 0)\begin{pmatrix} a & 0 & 0 \\ 0 & a & 0 \\ 0 & 0 & b \end{pmatrix}\begin{pmatrix} 1 \\ i \\ 0 \end{pmatrix}\right|^2 = \mathbf{0}$$

$$\mathbf{I_{\sigma^+\ in\ \sigma^-\ out}\,(E_g)} = \left|\frac{1}{2}\times\begin{pmatrix}1 & i & 0\end{pmatrix}\begin{pmatrix}c & 0 & 0\\ 0 & -c & d\\ 0 & d & 0\end{pmatrix}\begin{pmatrix}1\\ i\\ 0\end{pmatrix}\right|^2 +$$

$$\left|\frac{1}{2}\times\begin{pmatrix}1 & i & 0\end{pmatrix}\begin{pmatrix}0 & -c & -d\\ -c & 0 & 0\\ -d & 0 & 0\end{pmatrix}\begin{pmatrix}1\\ i\\ 0\end{pmatrix}\right|^2$$

$$= \left|\frac{1}{2}\times\begin{pmatrix}1 & i & 0\end{pmatrix}\begin{pmatrix}c\\ -ic\\ id\end{pmatrix}\right|^2 + \left|\frac{1}{2}\times\begin{pmatrix}1 & i & 0\end{pmatrix}\begin{pmatrix}-ic\\ -c\\ -d\end{pmatrix}\right|^2 = \mathbf{2|c|^2}$$

*Table T1: Selection rule for Raman-active phonons of $Fe_4GeTe_2$*

| | **$A_{1g}$ (Γ)** | **$E_g$ (Γ)** |
|---|---|---|
| $I_{linear\ \parallel}$ | $\lvert a\rvert^2$ | $\lvert c\rvert^2$ |
| $I_{linear\ \perp}$ | 0 | $\lvert c\rvert^2$ |
| $I_{\sigma+\ in\ \sigma+\ out}$ | $\lvert a\rvert^2$ | 0 |
| $I_{\sigma+\ in\ \sigma-\ out}$ | 0 | $2\lvert c\rvert^2$ |

**Section S2. $Fe_4GeTe_2$ single crystal growth, characterization, exfoliation and Raman measurement details**

*S2.1 $Fe_4GeTe_2$ single crystal growth:*

The high-quality single crystals of $Fe_4GeTe_2$ were grown using the standard chemical vapor transport (CVT) method, with $I_2$ as a transport agent. A mixture of highly pure (99.99%) Fe, Ge, and Te powders in a molar ratio of 5:1:2 was sealed in a high-vacuum quartz tube and heated at 725°C for seven days. The resulting material was reloaded into another evacuated quartz tube and placed in a horizontal two-zone furnace, with temperatures maintained at 800°C (hot end) and 750°C (cold end) for another seven days in the presence of $I_2$ (2 mg/cc). Thin single crystals were collected from the cold end, typically sized 1.3 × 1.3 × 0.05 $mm^3$. Detailed procedures are available in our earlier reports[1,2,3].

*S2.2 Crystal characterizations:*

X-ray diffraction (XRD) was performed on freshly cleaved, shiny $Fe_4GeTe_2$ single crystals[1]. Sharp (00l) peaks confirmed that the flat surface lies perpendicular to the crystallographic *c*-axis, with an interlayer spacing of 28.74 Å. High-resolution transmission electron microscopy (HRTEM) and energy-dispersive X-ray (EDX) spectroscopy verified good crystal quality. Atomic force microscopy (AFM) characterizations were carried out in tapping mode using a Cypher S AFM at room temperature under ambient conditions. Detailed sample preparation and characterization are also available in our earlier reports[1,2,3].

*S2.3 $Fe_4GeTe_2$ exfoliation:*

$Fe_4GeTe_2$ flakes were obtained using the scotch tape method from the high-quality bulk crystals. Polydimethylsiloxane (PDMS) stamps helped to isolate thinner flakes. Thickness of the flakes were initially determined via optical contrast and then confirmed by atomic force microscopy. The substrate was pre-cleaned ultrasonically with acetone, 2-propanol, and deionized water, followed by oxygen plasma cleaning to remove surface contaminants.

*S2.4 Raman measurements:*

Raman spectra were acquired using a LABRAM HR 800 spectrometer with an 80 cm focal length, 1800 gr/mm grating, a Peltier-cooled CCD detector, and a liquid-nitrogen cryostat (80–370 K). A 100X objective (NA = 0.9) focused a 488 nm $Ar^+$ laser onto an 80 nm $Fe_4GeTe_2$ flake (R80). For verification, the experiment was repeated using a 532 nm laser on a 190 nm thick flake across 83–370 K. A 50X long-working-distance objective (NA = 0.9, 721 nm spot size) was used. Laser power was kept below 250 μW, and each spectrum was recorded with a 90 s integration time. Temperature sweeps were conducted using a Linkam THMS600 stage, with closer steps near the spin reorientation temperature (SRT) and larger steps elsewhere. Polarization control was achieved with linear polarizers and a half-wave plate.

Low-temperature Raman (4–300 K) was performed in a Montana cryostat using a Renishaw inVia Raman system in backscattering geometry on the same 190 nm flake (R190), excited with a 532 nm laser and collected with a 2400 gr/mm grating. A 50X long-working-distance objective (NA = 0.5, 0.8 mm working distance) was used, with a spectral resolution of ~1 $cm^{-1}$.

*Table T2: Details of studied $Fe_4GeTe_2$ flakes for Raman measurements*

| Sample name | Thickness (nm) | Spectral ranges ($cm^{-1}$) | Grating used (g/mm) | Laser wavelength (nm) | Temperature range (K) | Measurements | See Sections |
|---|---|---|---|---|---|---|---|
| R190 | 190 | 50 - 1200 | 1800 | 532 | 80 - 370 | Temperature dependent | S6 |
| | | 100 - 600 | 2400 | 532 | 4 - 300 | Temperature dependent | S5 |
| R80 | 80 | 50 – 1200 | 1800 | 488 | 80 - 300 | Temperature dependent | S7 |
| R8 | 8 | 50 – 1200 | 1800 | 532 | 80 - 350 | Temperature dependent | S8 |
| - | ~ 9-10 nm to bulk | 50 - 600 | 1800 | 532 | 300 | Thickness dependent | S3 |
| - | 10 | 50 - 600 | 1800 | 532 | 300 | Room temperature | S9 |
| - | 14 | 50 - 600 | 1800 | 532 | 80 - 300 | Temperature dependent | S9 |
| - | 85 | 50 - 600 | 1800 | 532 | 300 | Laser power dependent | S4 |
| - | 9 | 50 - 600 | 1800 | 532 | 300 | Laser power dependent | S4 |

## Section S3. Thickness dependent Raman measurements

Raman spectroscopy is a powerful tool for determining the thickness of 2D materials due to its sensitivity to layer-dependent spectral changes[6–8]. As the layer number increases, the frequency of the primary Raman peaks either increases or decreases. For example, in transition-metal dichalcogenides (TMDCs)[9–11], the out-of-plane $A_{1g}$ mode increases in frequency (upshifts), while the in-plane $E_{2g}$ mode decreases in frequency (downshifts) with the increase in their thicknesses, reflecting interlayer interactions. The intensity and the peak positions of Raman signals serve as a reliable indicator of the material's thickness, making it highly useful for accurately identifying layer numbers in 2D materials.

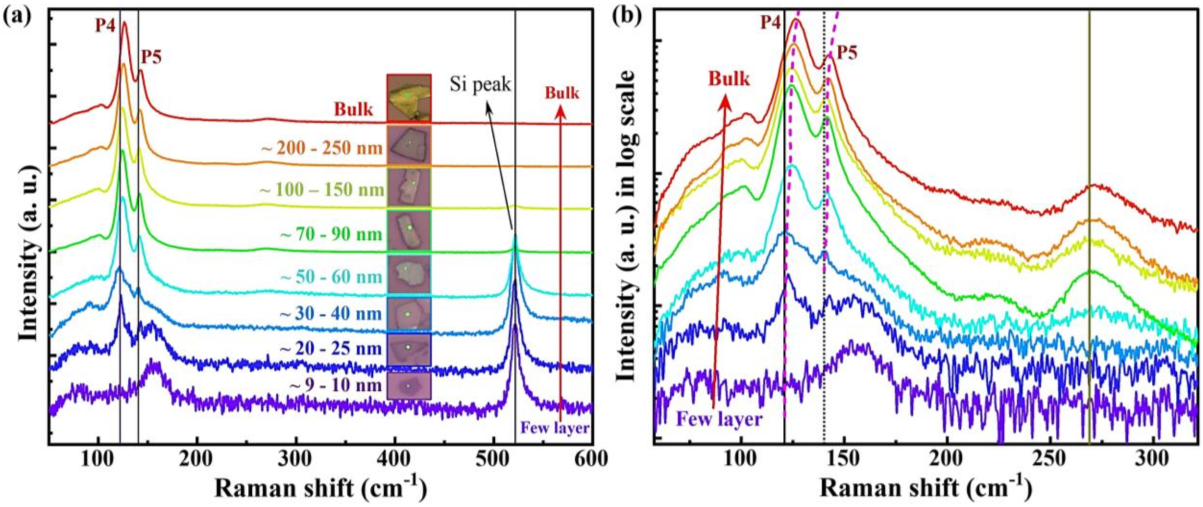


**Figure S1.** *(a) Thickness dependent Raman spectra from few layers to bulk $Fe_4GeTe_2$. The peaks P4 and P5 positions are shifting towards higher frequencies (blue-shift) with increasing thickness. Inset: Optical microscopic image of the flakes of $Fe_4GeTe_2$ and their approximate thickness estimated from the color contrast. (b) The thickness-dependent Raman spectra are plotted in a semi-logarithmic scale, for visual understanding of the shifting of the most intense peaks P4 and P5 with increasing thickness. The purple dotted lines are the guide to the eyes.*

Raman spectroscopy was performed on $Fe_4GeTe_2$ samples with varying thicknesses, from bulk crystal to few-layers, to examine layer-dependent changes. The samples were exfoliated using the mechanical exfoliation technique with Scotch tape. The thickness of analyzed $Fe_4GeTe_2$ flakes was determined using the optical contrast method[11–15], which involves placing the 2D material on a high-contrast substrate (here $Si/SiO_2$) and estimating layer numbers by comparing the color/contrast with the background. Figure S1(a) shows the Raman spectra of the exfoliated $Fe_4GeTe_2$ samples, highlighting the P4 and P5 peaks across different thicknesses. In bulk crystals, the P4 and P5 peaks exhibit higher intensity. As the layer count decreases, the intensity of both P4 and P5 peaks gradually reduces, and Si peaks near 520 $cm^{-1}$ start to enhance, as expected. In flakes thinner than 50 nm, a new broad peak around 160 $cm^{-1}$ begins to emerge. In 20-30 nm flakes, the coexistence of all three peaks is observed. With further reduction in thickness, this broad peak becomes more pronounced, while the intensities of the P4 and P5 peaks continue to decrease. In the thinnest measured flakes (9–10 nm), the P4 and P5 peaks completely vanished, leaving only the broad peak at the same position near 160 $cm^{-1}$. The gradual appearance of the broad peak is clearly observed in Figure S1(b). The emergence of

the broad peaks is probably due to the oxidation of the top layer in ambient atmosphere. As thinner layers are more prone to oxidation, the most pronounced broader peak is observed in the thinnest measured flake.

Additionally, as the thickness increases beyond 25 layers, both the P4 and P5 peaks exhibit a continuous frequency increase (blue shift) (see Figure S1(b)). This behavior mirrors what is typically observed in transition-metal dichalcogenides (TMDCs)[9–11], where the out-of-plane vibrational modes stiffen (upshift) and the in-plane modes soften (downshift) with increasing layer numbers. In this case, the P4 and P5 modes are mixed modes, consisting of a dominant out-of-plane vibrational mode with higher intensity and an in-plane vibrational mode with significantly lower intensity, as shown in Figures 1(e), (f) and Figure 2 (main text). As the number of layers increases, the contribution of the out-of-plane vibrational modes becomes more significant, resulting in a continuous increase in frequency. This result is also consistent with our previous report[2]. It is important to note that the laser power used for Raman spectroscopy measurements was maintained below 250 μW for all the layers to prevent laser-induced damage to the flakes, and all the measurements were performed in high vacuum.

Furthermore, we conducted temperature-dependent Raman measurements on the thinner flakes (≈ 8 nm) and observed no significant peak shifts as the temperature decreases from 300 K to 83 K (see Section S8 for details).

## Section S4. Laser power dependent Raman measurements under high vacuum

To examine the stability of unprotected $Fe_4GeTe_2$ flakes under laser irradiation, we conducted systematic, laser power-dependent Raman measurements at 300 K. Initially, we investigated a thicker $Fe_4GeTe_2$ flake (~ 85 nm). As the laser power was progressively increased from 12 μW to 4.5 mW, no observable shifts or new peaks appeared. However, we observed a systematic increase in the intensity of all peaks, particularly at ~104 $cm^{-1}$(P3), ~128 $cm^{-1}$(P4) and ~143.5 $cm^{-1}$(P5), along with an enhancement of the Si peaks, as expected (see Figure S2). Similar results were obtained when we repeated these measurements on other thick flakes (> 60 nm) (not shown). Therefore, we conclude that, similar to $Fe_3GeTe_2$[16], thick flakes of the 2D ferromagnet $Fe_4GeTe_2$ are relatively stable under atmospheric conditions and laser power.

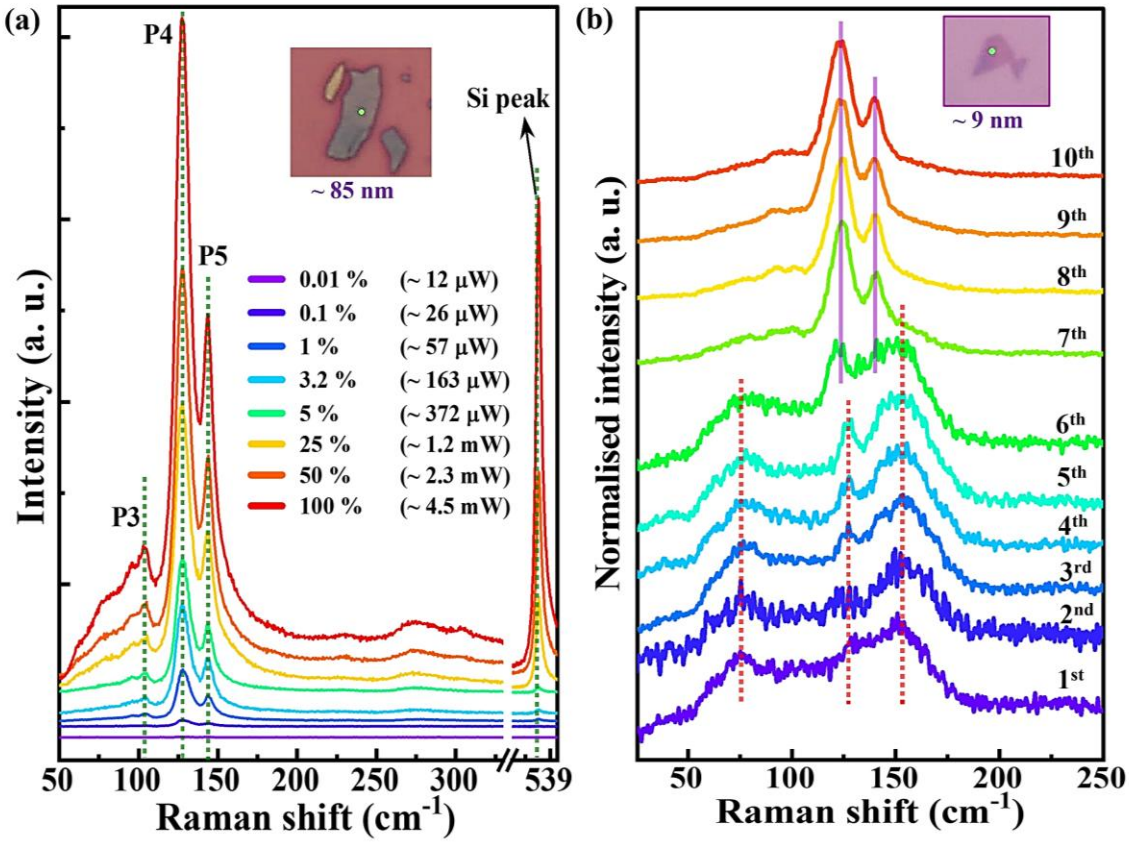


**Figure S2. (a)** *Laser power dependence of Raman spectra of a (a) multi-layer (~ 85 nm) and (b) few layer (~9 nm) flake of $Fe_4GeTe_2$ at 300 K with the same excitation source of 532 nm laser. Inset: The optical microscopy image the measured flakes where green dot is the position of the laser spot.*

For few-layer flakes (~ 9 nm), up to 700 μW, a broad Raman spectrum was observed, probably due to the surface oxidation of the thinner flakes, and this remained unchanged even after successive measurements at the same location. Furthermore, to investigate laser radiation-induced removal of the oxidation layer in the few-layer flakes, we applied a relatively high laser power (~ 4.7 mW) to a thinner flake (~ 9 nm) and monitored the Raman spectra at the same spot to track any signs of getting back to the original signal. Interestingly, we found that relatively higher laser radiation could induce the removal of the oxidation layer in the unprotected thinner flakes.

Figure S2 presents a series of Raman spectra measured continuously under this higher laser power. With successive measurements, the three phonon modes of $Fe_4GeTe_2$ (probably due to oxidation of the top layer in ambient atmosphere) gradually disappeared (red dotted lines), while two expected phonon modes emerged near 123 $cm^{-1}$ and 140 $cm^{-1}$ (purple solid lines). The emergence of these two modes occurs at different positions (approximately 5 (P4) and 3 $cm^{-1}$ (P5) apart, see Figure S3) compared to the positions of P4 and P5 of the multilayer flakes, as expected, due to the shifting of the peak positions with reducing thickness (see Figure S1(b)). While the exact origin of these three broadened peaks requires further study, the re-appearance of the two Raman modes (P4 and P5) during the exposure to the laser power in $Fe_4GeTe_2$ provides a straightforward and efficient method for assessing the $Fe_4GeTe_2$ thinner flakes. This characteristic offers $Fe_4GeTe_2$ a unique advantage over other 2D ferromagnetic materials, such as $Fe_3GeTe_2$, $Cr_2Ge_2Te_6$, $CrI_3$, etc.[16–19] which degrade rapidly in atmospheric conditions, thereby facilitating both future fundamental research and potential applications.

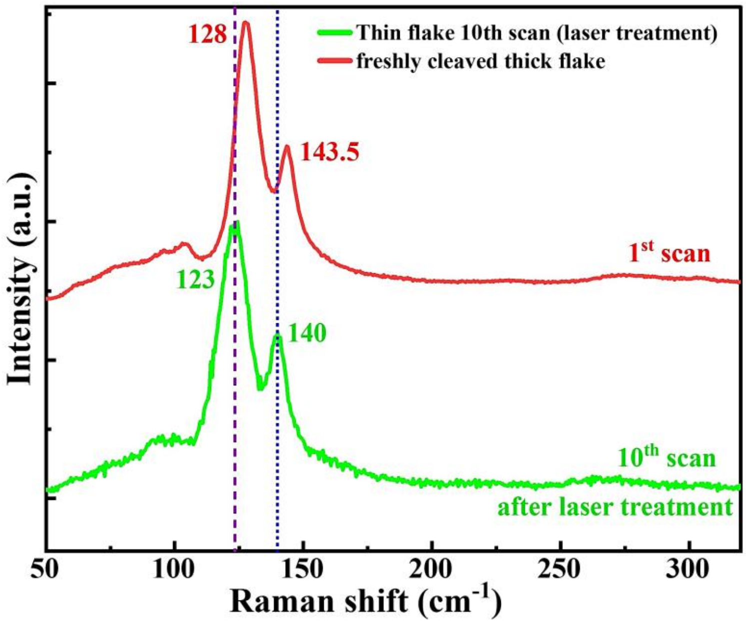


**Figure S3.** *Comparison of the Raman spectra of a freshly exfoliated multi-layer flake (~ 85 nm) (red curve) and the laser treated few-layer (~9 nm) flake (green curve) of $Fe_4GeTe_2$ at 300 K with the same excitation source of 532 nm laser with the same laser power.*

## Section S5. Low temperature (down to 5 K) Raman measurements of R190

*S5.1 Comparison of Raman spectra with previous measurements:*

To further investigate the low-temperature evolution of the Raman spectra of the same flake R190, we conducted temperature-dependent Raman measurements from 300 K down to 4 K using a Montana cryostat integrated with a Renishaw inVia Raman spectrometer in a backscattering configuration. A 532 nm laser was used for excitation, in combination with a 2400 g/mm grating. The Raman signal was collected using a 50X long working distance objective (0.8 mm working distance, numerical aperture NA = 0.5). The spectral resolution of the system was approximately 1 $cm^{-1}$. However, the acquired spectra covered a range starting

from 100 $cm^{-1}$, instead of the previously acquired spectra from 50 $cm^{-1}$ on $LN_2$ (77 K) setup. While the peak positions remained consistent, the P4 and P5 peaks exhibited broadening compared to earlier measurements, as compared at the similar temperatures (see Figure S4).

The observed constant broadened peaks (P4 and P5) at room temperature to the low temperature could be attributed to several factors. Given that this measurement was performed several days after the initial ones, the flake may have degraded over time, leading to peak broadening, despite being stored in an inert atmosphere inside a glovebox. Additionally, the use of a low-resolution setup can contribute to the observed broadening and a constant peak position shifting, as instrumental resolution plays a crucial role in accurately resolving closely

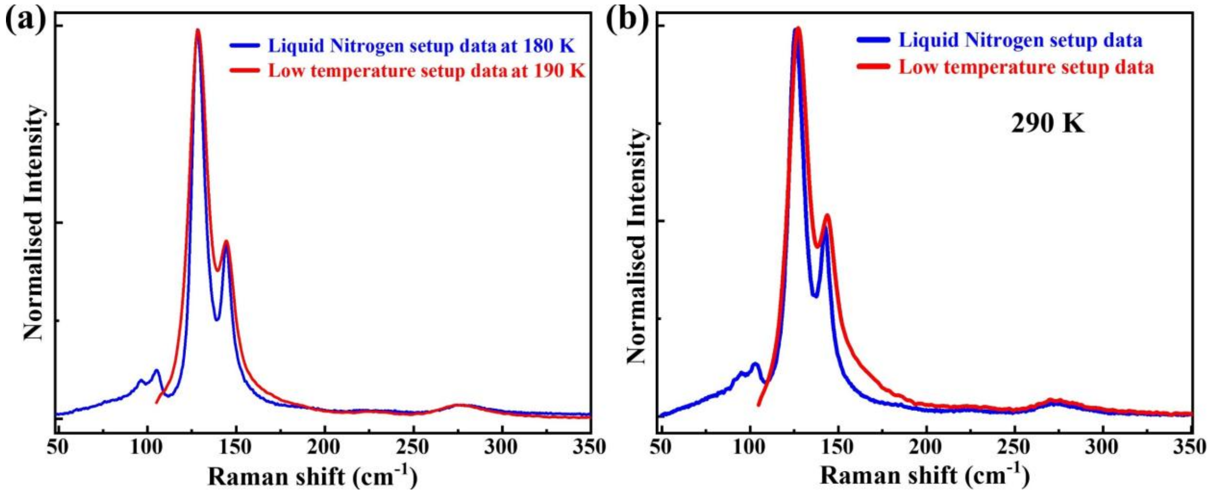


**Figure S4.** *Comparison of the Raman data in two different setups, one in a high-resolution liquid $N_2$ (~ 80 K) setup with spectrum starting from 50 $cm^{-1}$ as indicated by blue curve, and another in a low-resolution low-temperature (~ 5 K) setup with spectrum starting from 100 $cm^{-1}$ indicated by red curve. The comparison is shown (a) at ~ 180 K and (b) at ~ 290 K.*

spaced spectral features. For our case, the peak positions for both peaks P4 and P5 are shifted slightly to the higher frequency at 290 K, but matches with the previous data at T ~ 180-190 K. However, it shows a similar and consistent behaviour like $LN_2$ setup. It's also important to consider that the reduced spectral range (starting from 100 $cm^{-1}$ instead of 50 $cm^{-1}$) may exclude low-frequency modes that could influence the overall spectral analysis. Therefore, the experimental conditions and the flake degradation can be responsible for the observed spectral changes.

*S5.2 Fitting of Raman data with multi-Lorentzian functions:*

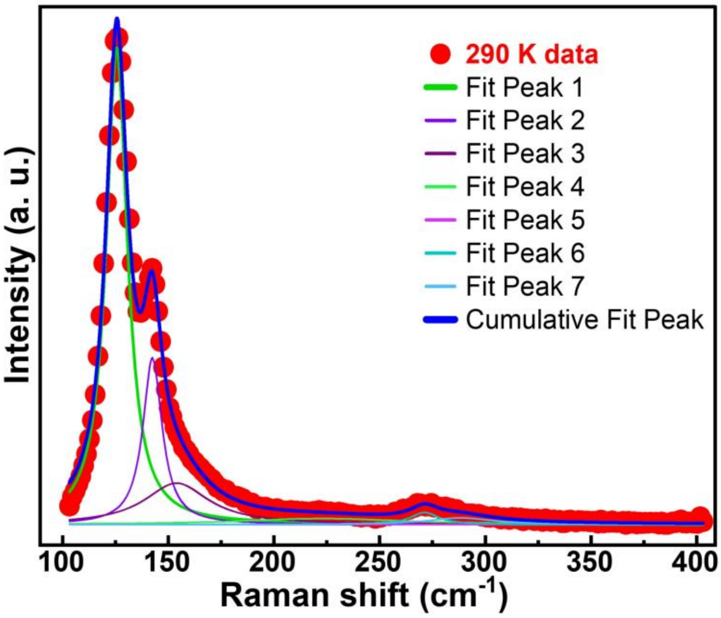


**Figure S5.** *Fitting of the 290 K Raman Spectra with eight Lorentzian functions*

Figure S5 shows the multi-Lorentzian fitting of the Raman spectrum of the R190 flake measured at 290 K using the low-temperature setup down to 5 K. The cumulative fit includes a total of seven distinct peaks (P4–P10) above 100 $cm^{-1}$, confirming that these modes provide the best fit for the observed spectrum and accurately capture its features. Among them, P4 and P5 exhibit the most prominent signals, consistent with previous measurements. Additionally, P9 and P10 show relatively stronger signals compared to the remaining peaks.

*S5.3 Temperature dependent Raman spectra:*

Figure S6 shows the full temperature-dependent Raman spectra of the R190 flake, recorded across the 5 K to 300 K range, with particular focus on the evolution of the P4 and P5 peaks. A visual inspection reveals a similar temperature-dependent behavior of these peaks as previously observed in the LN2 setup. To ensure accurate analysis, we performed multi-Lorentzian fitting of the spectra at all measured temperatures, following the same procedure used for the 290 K data (see Figure S5). From these fits, $\omega_{ph}$ and $\Gamma_{ph}$ were extracted for P4 and P5 modes and plotted as a function of temperature, as shown in Figure S7.

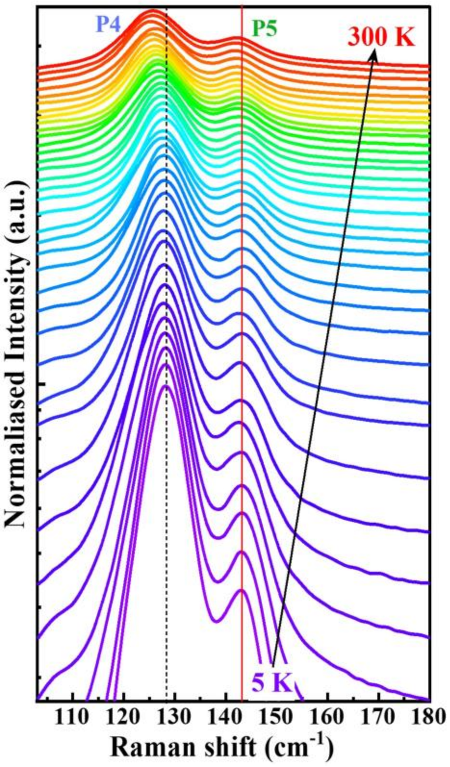


**Figure S6.** *Temperature-dependent Raman spectra at different temperatures from 300 K down to 5 K.*

*S5.4 Temperature dependence of $\omega_{ph}$ and $\Gamma_{ph}$ of P4 and P5 down to 5 K*

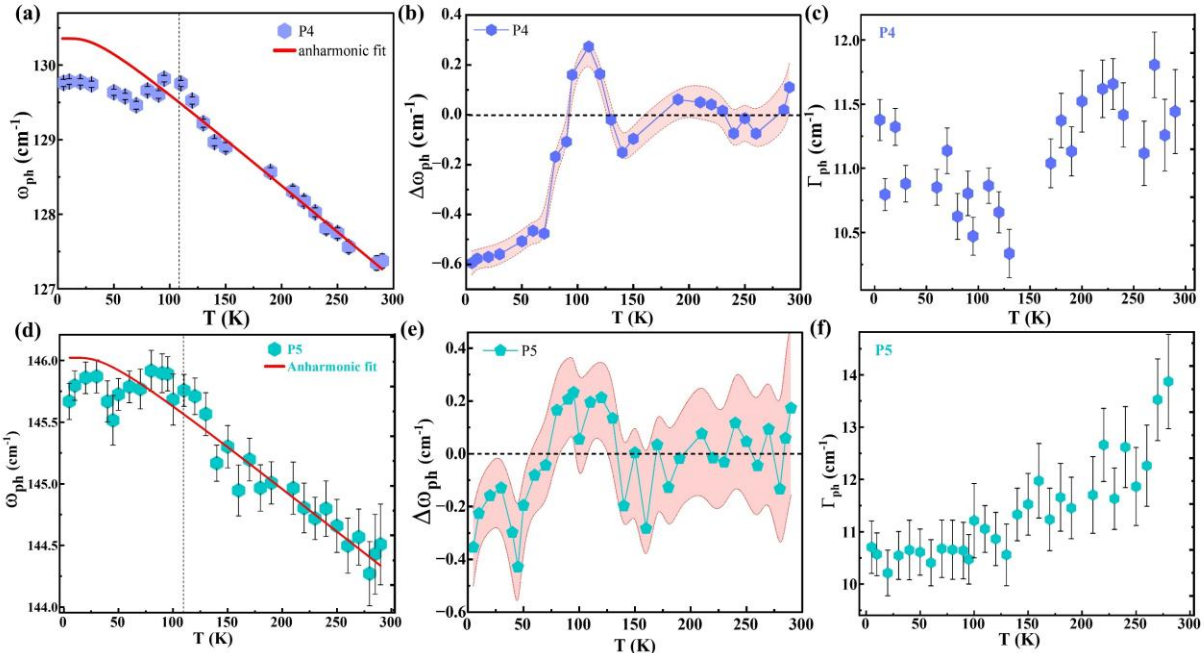


**Figure S7.** *(a), (d) The temperature dependence of the phonon frequencies (peak positions) for the Raman modes, P4 and P5, respectively for R190 flake. These data points are fitted with standard anharmonic model (red fitted lines). (b), (e) The deviation of the phonon frequencies from the anharmonic model is plotted against temperature for these two modes. Red areas indicate the error bars. (c), (f) The temperature-dependent phonon linewidths (FWHM) for the corresponding modes.*

Figure S7 represents the temperature-dependent evolution of the phonon frequencies ($\omega_{ph}$) and linewidths ($\Gamma_{ph}$) for the Raman modes P4 and P5 for the R190 flake, measured over a range from 5 K to 300 K. The extracted phonon frequencies for both modes are fitted using the standard anharmonic model (indicated by red fitted lines, Figure S7(a), (d)), which accurately describes the high-temperature phonon behavior. However, as the temperature decreases below $T_{SR}$, clear deviations from this model are observed (similar to Figure S13), indicating the influence of spin-phonon coupling. These deviations are plotted separately in Figure S7 (b), (e) for both modes to highlight the anomalous behavior, with shaded red regions representing the error margins. In addition to the frequency shifts, the corresponding phonon linewidths (FWHM) for P4 and P5 also exhibit distinct temperature dependence below and above SRT, consistent with enhanced phonon-spin interactions at low temperatures. However, the spectra from the low-temperature setup exhibit broader linewidths and increased error bars, highlighting the difficulty in extracting precise temperature-dependent linewidths under such conditions. A comparative analysis of the extracted FWHMs shown in Figure S8 reveals that the low temperature setup yields significantly larger uncertainties than the liquid nitrogen setup, emphasizing the spectral resolution and minor flake degradation as explained in Section S5.1.

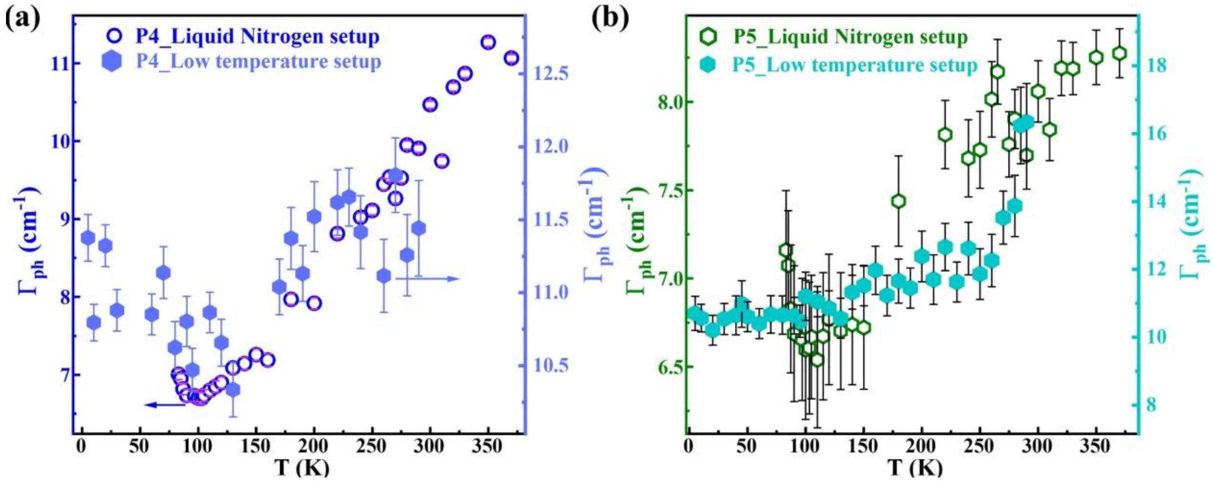


**Figure S8.** *The comparison of the temperature dependence of the linewidths (FWHMs), for the Raman modes, (a) P4 and (b) P5, respectively with the measurements in two different setups. The low temperature setup data shows the error bars are larger compared to the liquid $N_2$ setup data for P4 mode.*

## Section S6. Additional Raman data and analysis of R190

*S6.1 Raman data in full spectral range for R190:*

We have performed the Raman measurement for R190 in the spectral range of 50 - 1200 cm$^{-1}$ at 300 K (as shown in Figure S9(b)). The AFM height profile (Figure S9(a)) shows that the thickness ~ 190 nm. The integration time for each Raman spectrum was set to 90 seconds. The full range spectrum reveals several peaks below 400 cm$^{-1}$ from the flake, while characteristic Si peaks are observed near 521 cm$^{-1}$ and in between 935–990 cm$^{-1}$ (Figure S9(b) inset), in the higher frequency range. The presence of Si peaks suggests that the Raman signal is originating

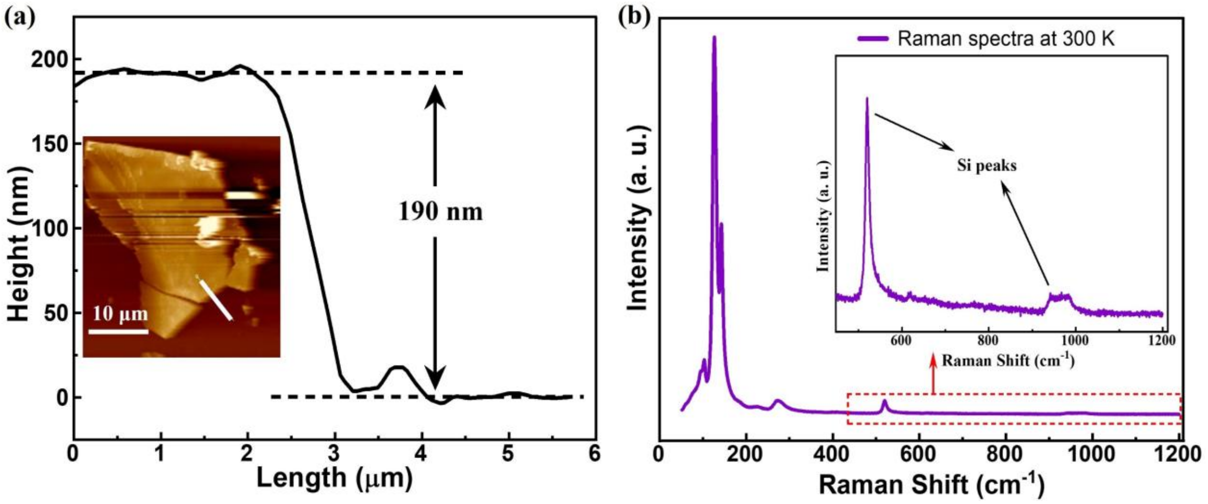


**Figure S9.** *(a) Height profile with standard AFM image of the R190 flake. (b) Full range Raman spectra from 50 cm$^{-1}$ to 1200 cm$^{-1}$ at 300 K with the excitation source of 532 nm laser. Inset: Peaks corresponding to Si are only observed near 521 cm$^{-1}$ and 935-990 cm$^{-1}$, in the high frequency spectral ranges above 400 cm$^{-1}$.*

not only from the top surface of the flake but, more importantly, from R190 flake itself and the underlying Si/$SiO_2$ substrate.

*S6.2 Fitting Raman data with multi-Lorentzian functions:*

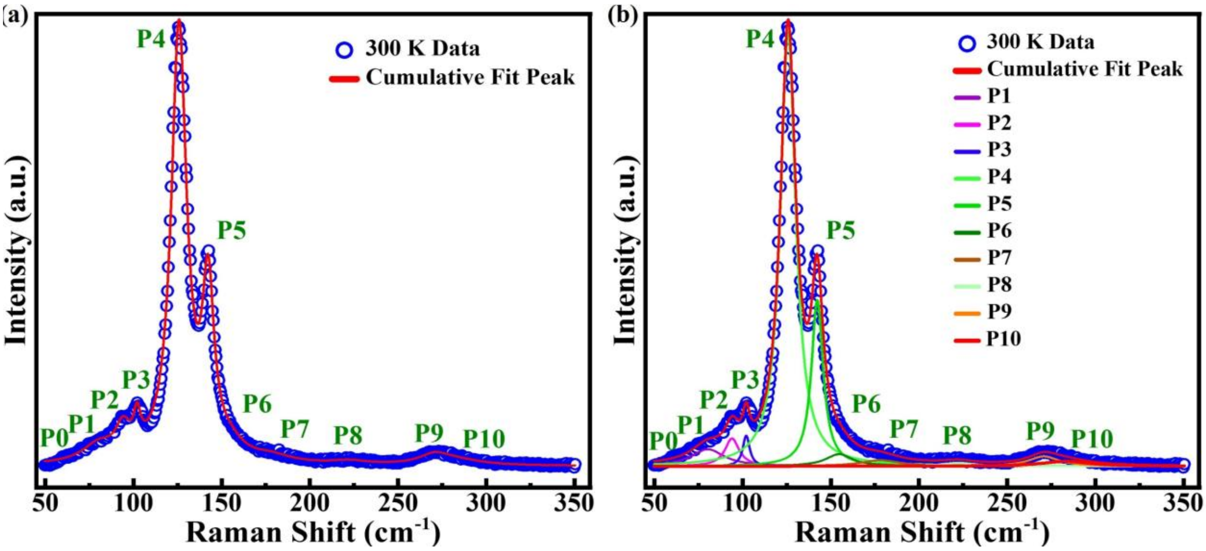


**Figure S10.** *(a) Raman spectrum of 190 nm thick flake with the cumulative fit at 300 K consisting of 11 peaks, P0-P10. (b) The multi-Lorentzian fitting reveals that a total of 11 peaks provide the best fit for the observed spectra.*

Figure S10(a) presents the Raman spectrum of R190 flake measured at 300 K, showing the cumulative fit of the total 11 distinct peaks labelled by P0–P10. In Figure S10(b) the multi-Lorentzian fit confirms that these 11 peaks provide the best fit for the observed spectra, accurately capturing the spectral features. Among these peaks, P4 and P5 exhibit the most prominent signals. Additionally, P2, P3, P9, and P10 produce relatively stronger signals compared to the remaining peaks.

*S6.3 Temperature dependence of the less intense Raman modes:*

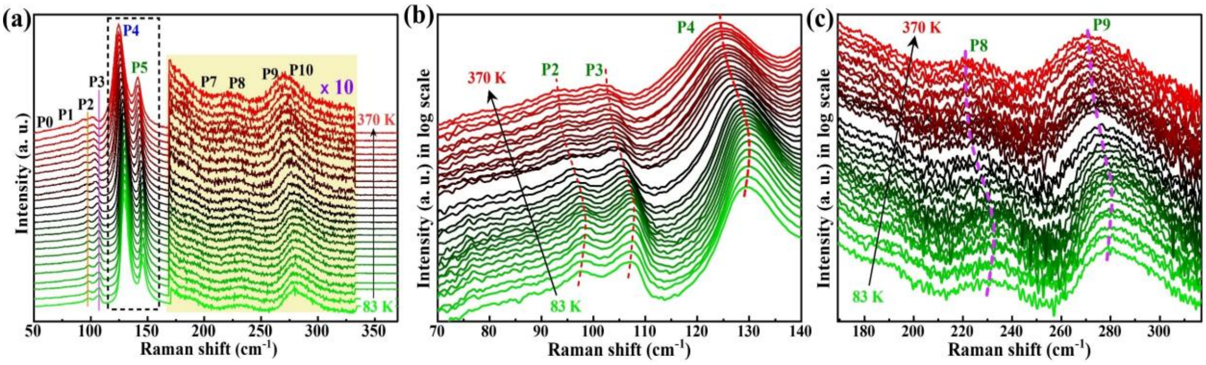


**Figure S11.** *Temperature dependent Raman spectra of R190 from 83 K to 370 K focussing (a) all the peaks (b) the peaks P2, P3 and P4, (c) P8 and P9. Red and pink dashed lines are guide to eye.*

Figure S11(a) presents the temperature-dependent Raman spectra of R190 flake, recorded over a temperature range of 83 K to 370 K. The spectra specifically highlight the evolution of peaks (b) P2, P3, and P4, and (c) P8 and P9. To better visualize the variations in peak intensity with temperature, the intensity axes are plotted on a logarithmic scale. From a visual inspection, we observe a temperature-dependent trend in P2, P3, and P4, as well as in P8 and P9, that is similar to the behavior of P4 and P5 discussed in the main text.

*S6.4 Temperature dependence of $\omega_{ph}$, $\Gamma_{ph}$ and Intensity of the less-intense Raman modes:*

The temperature dependence of $\omega_{ph}$, $\Gamma_{ph}$, and Intensity for the less intense peaks P1, P2, P3, and P9 for R190 are presented in Figure S12. Despite their lower intensity, all these peaks exhibit a similar trend with temperature. To ensure accurate analysis, we performed multi-Lorentzian fitting of the spectra at all measured temperatures, following the same procedure used for the 300 K data (Figure S10(b)). From these fits, $\omega_{ph}$ and $\Gamma_{ph}$ were extracted for P1, P2, P3, and P9 modes and plotted as a function of temperature, as shown in Figure S12. However, due to their weaker signal strength, the associated error bars are comparatively larger, indicating greater uncertainty in the extracted parameters.

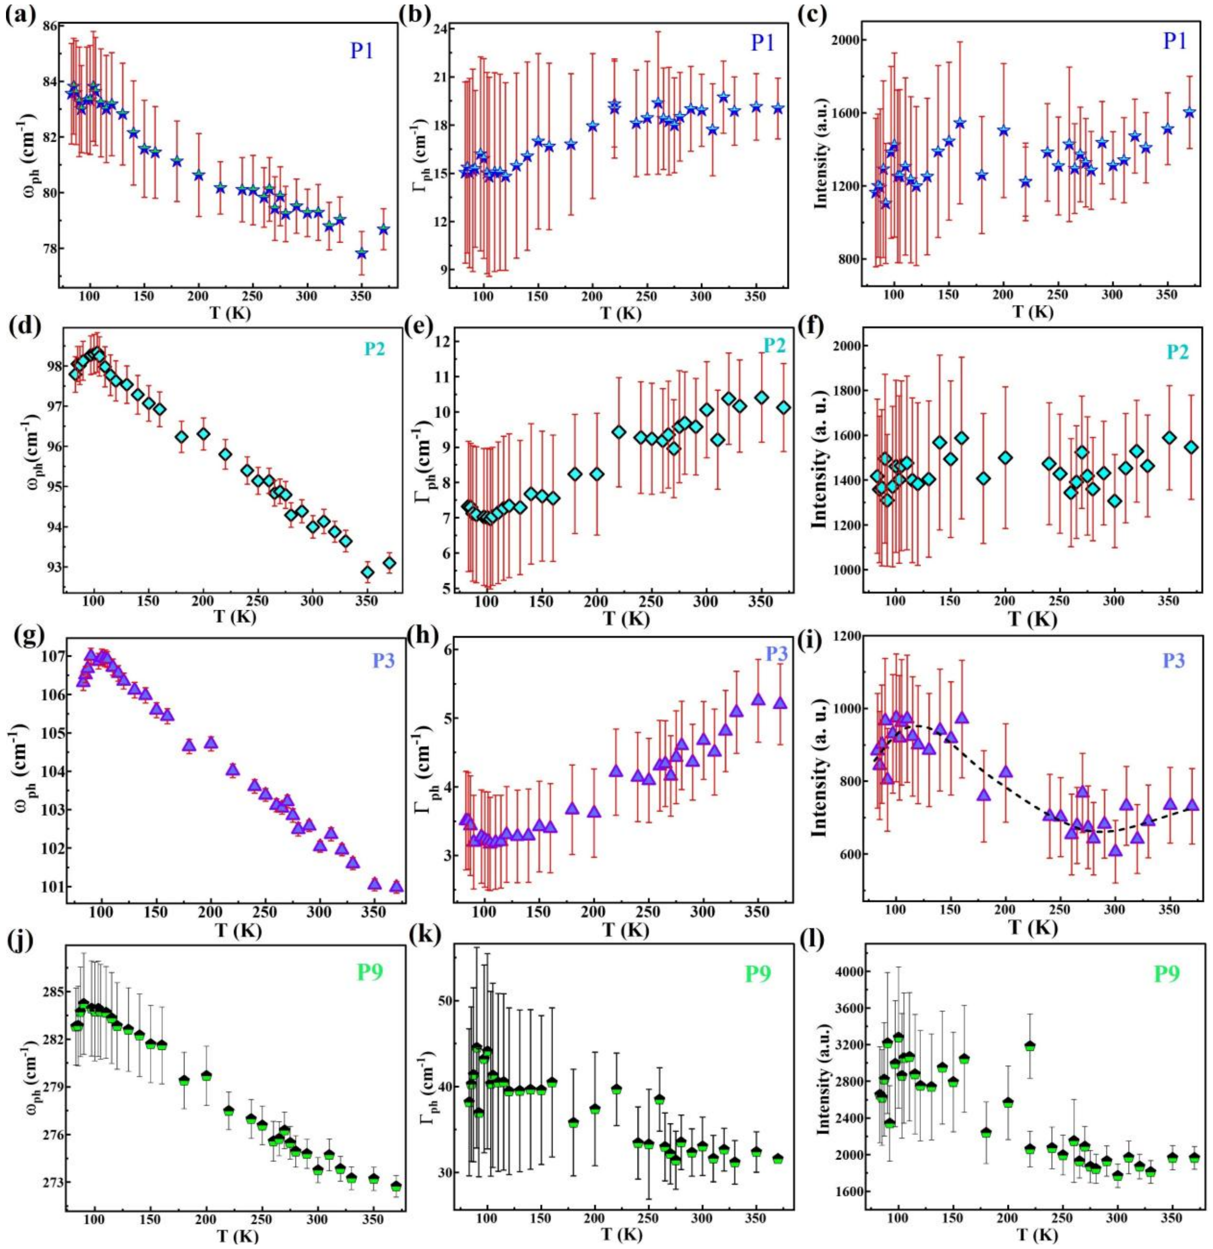


**Figure S12.** *Temperature dependence of* $\omega_{ph}, \Gamma_{ph}$ *and Intensity for the less intense peaks P1, P2, P3 and P9 of R190. All of them shows similar behaviour with temperature, though the error bars are larger for them.*

*S6.5 Temperature dependence deviations of $\omega_{ph}$ and $\Gamma_{ph}$ of the less-intense Raman modes, P2 and P3:*

The temperature-dependent $\omega_{ph}$ and $\Gamma_{ph}$ data for the two Raman modes (P2 and P3) were fitted using the standard anharmonic model (Eqns. 3 and 4 in the main text) over the temperature range of 120 K to 300 K, as plotted in Figure S13. Below $T_{SR}$, P2 and P3 modes (also P1 and P9 in Figure S12) exhibit clear deviations from the behavior predicted by the anharmonic model, as indicated by the red fit lines, similar to the deviations observed for modes P4 and P5 in the main text. These deviations are also plotted here for comparison in Figure S13.

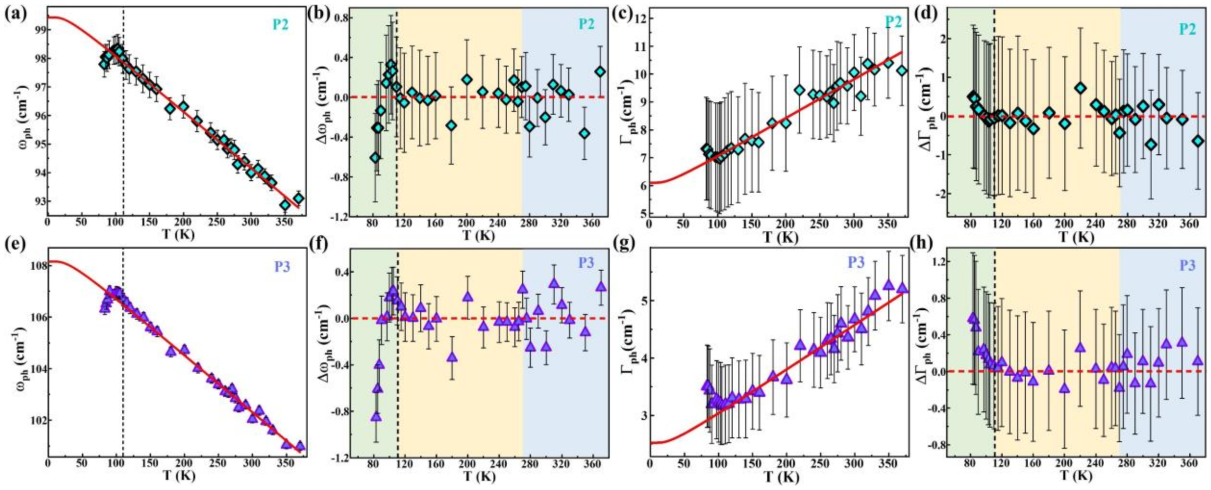


**Figure S13.** *Temperature dependence of* (**a**), (**c**) $\omega_{ph}$ *and* (**e**), (**g**) $\Gamma_{ph}$ *for P2 and P3 of R190 flake are fitted with standard anharmonic model (red curve). The corresponding deviations from the standard anharmonic model,* (***b***), (***f***) $\Delta\omega_{ph}$ *and* (***d***), (***h***) $\Delta\Gamma_{ph}$, *are observed below $T_{SR}$ for both P2 and P3, respectively.*

*S6.6 Temperature dependence of lifetime (τ) of phonons:*

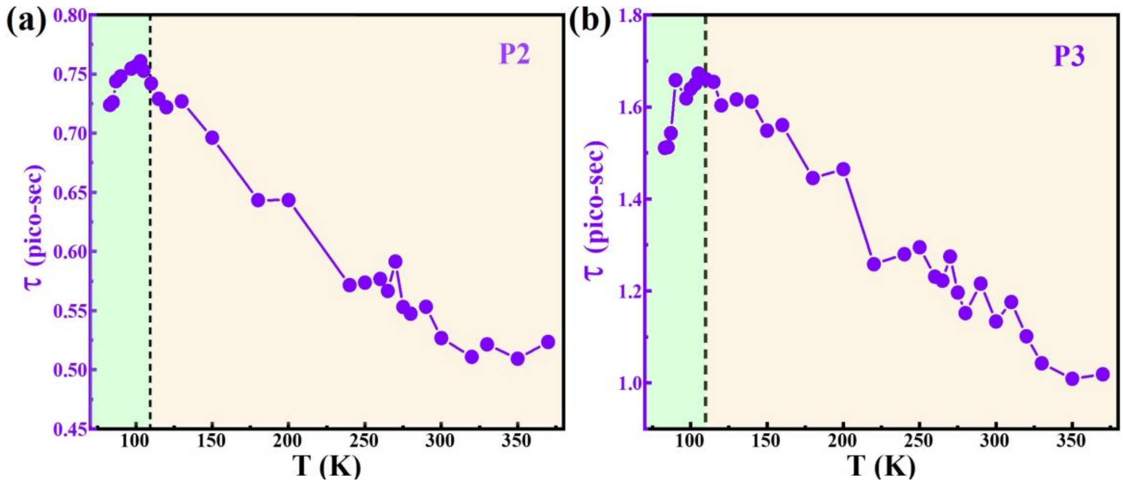


**Figure S14.** *The temperature dependence of $\tau$ for the modes P2 and P3 of R190 flake also, shows significant changes around $T_{SR}$ and $T_C$*

The presence of spin-phonon coupling is further supported by the analysis of phonon lifetimes ($\tau$), which are inversely related to the phonon linewidths ($\Gamma(T)$), as discussed in the main text. For modes P2 and P3 also, a clear trend is observed (see Figure S14): the phonon lifetime decreases with decreasing temperature below and above $T_{SR}$, mirroring the behavior observed for the P4 and P5 modes plotted in the main text.

*S6.7 Extraction of spin-phonon coupling strength ($\lambda_{s\text{-}ph}$):*

To estimate the interaction strength between the lattice vibrations and spin degrees of freedom, commonly referred to as spin-phonon coupling, one can utilize the relationship that connects phonon energy shifts to spin-spin correlations. The phonon frequency ($\omega_{ph}$) in a magnetic material is altered from its reference value in the absence of magnetic interactions ($\omega_0$) due to the coupling with local magnetic moments. This change is captured by the following approximated relation[20,21]:

$$\omega \approx \omega_0 + \lambda_{s\text{-}ph} \langle \mathbf{S_i} \cdot \mathbf{S_j} \rangle \ldots\ldots\ldots\ldots\ldots\ldots\ldots\ldots\ldots\ldots(S1)$$

Here, $\lambda_{s\text{-}ph}$ represents the spin-phonon coupling constant, and $\langle \mathbf{S_i} \cdot \mathbf{S_j} \rangle$ denotes the spin-spin correlation function of the neighboring spins. The parameter $\lambda_{s\text{-}ph}$ is inherently linked to the sensitivity of the exchange interaction J with respect to atomic displacements u, such that $\lambda_{s\text{-}ph} \propto \partial \mathbf{J}/\partial u \cdot \mathbf{u}$. Reorganizing the above expression, the strength of spin-phonon interaction can be approximated as:

$$\lambda_{s\text{-}ph} \approx (\omega - \omega_0)/\langle \mathbf{S_i} \cdot \mathbf{S_j} \rangle \ldots\ldots\ldots\ldots\ldots\ldots\ldots\ldots\ldots\ldots(S2)$$

To evaluate the spin-spin correlation function, we relate it to the magnetic moment using the known relation:

$$\mu = -g_s \mu_B \mathbf{S}$$

Given $g_s = 2$ for electrons, this implies: $S = -\mu/(2\mu_B)$. Thus, the spin-spin correlation can be estimated as:

$$\langle \mathbf{S_i} \cdot \mathbf{S_j} \rangle \approx (\langle \mu \rangle / 2\mu_B)^2 \ldots\ldots\ldots\ldots\ldots\ldots\ldots\ldots\ldots\ldots(S3)$$

We must admit that $Fe_4GeTe_2$ is a noncollinear ferromagnet and no theoretical calculations are currently available to predict this value. Therefore, this estimate is indeed crude. Based on magnetization measurements at 83 K, the average saturation magnetic moment per Fe atom is estimated to be approximately 1.827 $\mu_B$, corresponding to a reduced spin correlation value:

$$\langle \mathbf{S_i} \cdot \mathbf{S_j} \rangle \approx (1.827/2)^2 \approx 0.834$$

At this temperature, the P4 phonon mode exhibits a frequency shift of $\Delta\omega \approx 0.795\ cm^{-1}$. Substituting this value into the above Eqn. S2 yields spin-phonon coupling strength for P4 mode at 83 K as:

$$\lambda_{s\text{-}ph}\ (83\ K) = \Delta\omega_{ph}/\langle \mathbf{S_i} \cdot \mathbf{S_j} \rangle \approx 0.795/0.8345 \approx 0.95\ cm^{-1}$$

These calculations (see Table T3 as following) underscore the strong sensitivity of the spin-phonon coupling to both magnetic ordering and temperatures, highlighting its critical role in the magneto-lattice dynamics of $Fe_4GeTe_2$.

**Table T3**

| T (K) | ⟨μ⟩ ($\mu_B$/Fe) | ⟨$S_i \cdot S_j$⟩ | P4 | | P5 | |
|---|---|---|---|---|---|---|
| | | | $\Delta\omega_{ph}$ ($cm^{-1}$) | $\lambda_{s\text{-}ph}$ ($cm^{-1}$) | $\Delta\omega_{ph}$ ($cm^{-1}$) | $\lambda_{s\text{-}ph}$ ($cm^{-1}$) |
| 83 | 1.83 | 0.83 | 0.80±0.02 | 0.95±0.02 | 0.62±0.08 | 0.74±0.08 |
| 110 | 1.75 | 0.77 | 0.03±0.02 | 0.05±0.02 | 0.18±0.09 | 0.23±0.09 |

## Section S7. Temperature dependent Raman measurements of 80 layered flake (R80) of $Fe_4GeTe_2$

*S7.1 Fitting of Raman data with multi-Lorentzian functions:*

To validate our results, we have performed the temperature dependent Raman measurement in the spectral range of 50 - 1200 $cm^{-1}$ in another thick flake of $Fe_4GeTe_2$ but having much lower thickness ~ 80 nm (R80) (see AFM height profile, Figure S15 (a)). We obtained these flakes by mechanically exfoliating bulk crystals onto Si/$SiO_2$ substrates. Following exfoliation, we immediately placed our sample within a high vacuum sample holder to prevent oxidation of the flakes in the ambient atmosphere. All measurements were conducted under this vacuum condition, employing a liquid nitrogen flow cryostat with a temperature range of 80 - 300 K. The data were taken in a backscattering configuration using a 100x objective with a numerical aperture (NA) of 0.9 dispersed by 1800 g/mm grating and by using 488 nm wavelength beam from an air-cooled argon-ion laser. The Raman spectra was collected without any polarization configuration to get a better signal to noise ratio.

The analysis of the measured spectra involved deconvolution using multiple Lorentzian curves, enabling the identification of the minimum number of spectral components required to accurately represent the experimental spectrum. Similar to the R190 flake, the fitting process

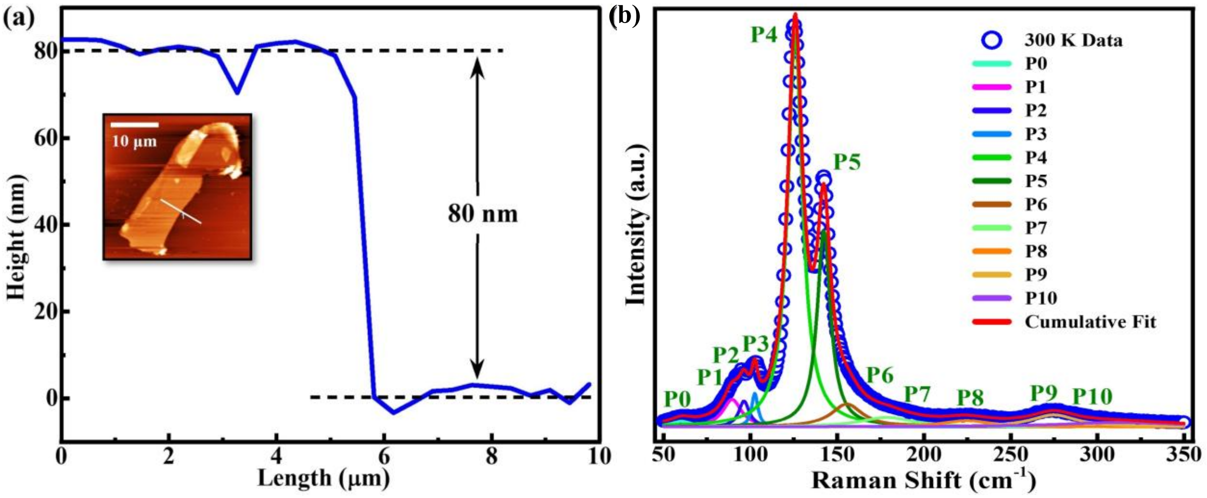


**Figure S15.** *(a) Height profile of the $Fe_4GeTe_2$ flake R80 measured by AFM. Inset: Atomic force micrograph of the flake. (b) The room temperature (300 K) Raman spectra (blue circles) ($\lambda_{ex}$ ~ 488 nm) of the flake are fitted with eleven Lorentzian functions, providing eleven Raman modes (P0-P10) and the fitted curve is indicated in red color.*

revealed eleven Raman modes (at 300 K), labelled as P0 to P10 within the spectral range of 50 - 350 $cm^{-1}$, as illustrated in Figure S15 (b). It should be noted that, similar to R190, no peaks are observed in the experimental data within the spectral range of 350 - 1200 $cm^{-1}$.

Detailed fitting results are shown in Figure S15 (b), where eleven Lorentzian curves combine to match the cumulative fit of the Raman spectra measured at 300 K. Among these eleven modes, four are the most intense: P2 (≈ 93 $cm^{-1}$), P3 (≈ 102.5 $cm^{-1}$), P4 (≈ 125.4 $cm^{-1}$), and P5 (≈ 142 $cm^{-1}$). Additionally, seven extremely weak kinks were observed at approximately 60.3 $cm^{-1}$ (P0), 83 $cm^{-1}$ (P1), 155 $cm^{-1}$ (P6), 179 $cm^{-1}$ (P7), 224 $cm^{-1}$ (P8), and 272 $cm^{-1}$ (P9), 284 $cm^{-1}$ (P10) in the experimental Raman spectra. It has been confirmed that excluding these seven weak peaks does not significantly affect the peak positions and the full width at half maximum

(FWHM) of the most intense peaks (P2-P5). However, their contributions were incorporated during spectrum analysis to enhance the reliability of the fitting process (see Figure S15 (b)). For a better understanding of the lattice dynamics and spin-phonon coupling in the $Fe_4GeTe_2$ crystal, we focus primarily on the most intense peaks (P2-P5), as they show significant changes with temperature and different configurations compared to the less intense peaks.

**Table T4: Peak positions of the Raman modes in the Raman spectra**

| Peak Names | **P0** | **P1** | **P2** | **P3** | **P4** | **P5** | **P6** | **P7** | **P8** | **P9** | **P10** |
|---|---|---|---|---|---|---|---|---|---|---|---|
| Peak positions ($cm^{-1}$) | 60.3 | 83 | 93 | 102.5 | 125.4 | 142 | 155 | 179 | 224 | 272 | 284 |

*S7.2 Temperature dependent Raman spectra:*

To delve deeper into the lattice dynamics, we performed a temperature-dependent Raman study on this R80 flake of $Fe_4GeTe_2$ crystal, covering a temperature range from 83 to 300 K. The Raman spectra obtained at various temperatures are shown in Figure S16 and S17. The Raman-active modes P4-P5 exhibit significant broadening and softening as the temperature rises above approximately $T_{SR}$ (~ 110 K), as clearly seen in the semi-logarithmic plot in Figure S17(b). Starting from 83 K, the peak positions initially show a continuous blueshift up to $T_{SR}$. However, above $T_{SR}$, an unusual redshift is observed, extending up to 300 K. To accurately analyse the temperature-dependent Raman data, we applied multi-Lorentzian functions to fit

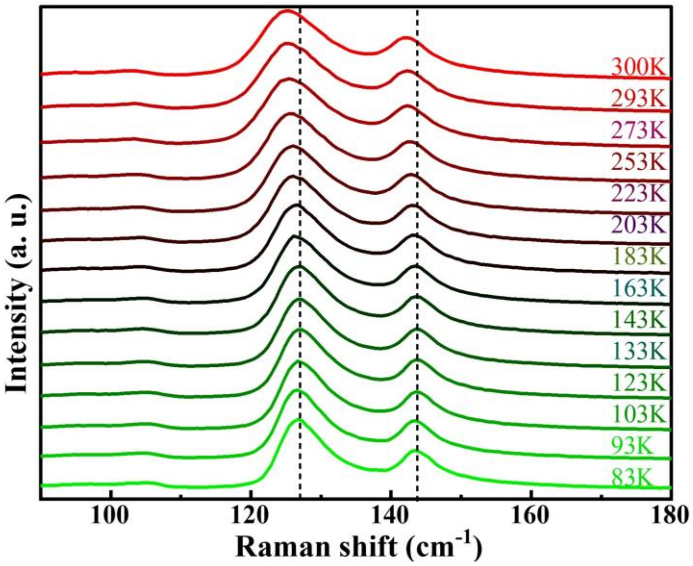


**Figure S16.** *Temperature-dependent Raman spectra in the increment plot at different temperatures down to 83 K.*

the spectra at all measured temperatures, using a similar approach as shown in Figure S15(b).

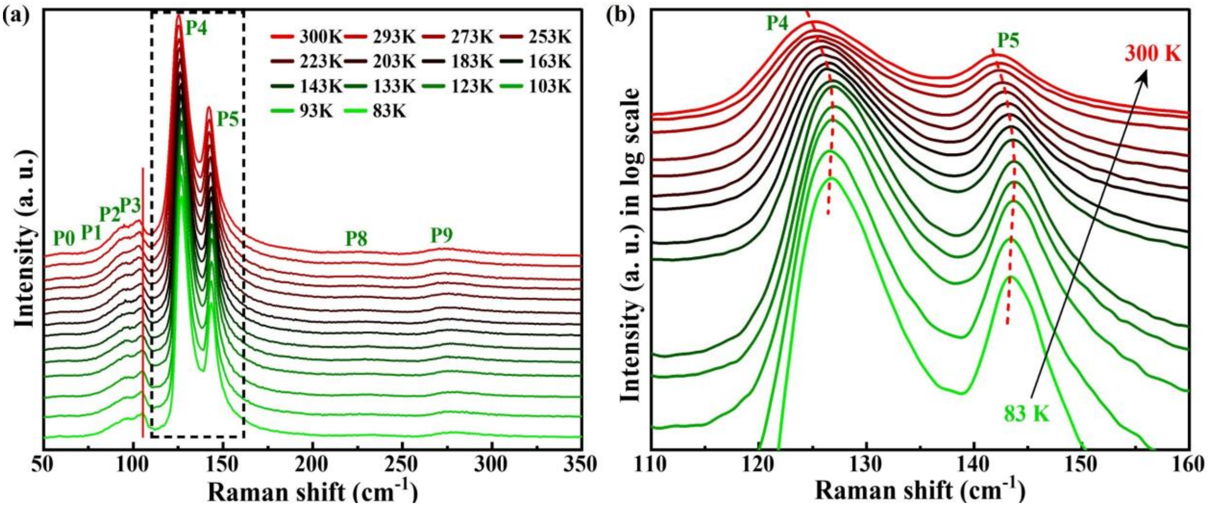


**Figure S17.** *(a) Temperature-dependent Raman spectra at different temperatures down to 83 K. The peaks are named sequentially P0-P10. The black rectangular box indicates the two most intense peaks, P4 and P5. The red line indicates the shifting of the peak P3 with temperature. (b) The temperature-dependent Raman spectra are plotted in a semi-logarithmic scale, for visual understanding of the shifting of the most intense peaks P4 and P5 with temperature. The red dotted line is a guide to the eye.*

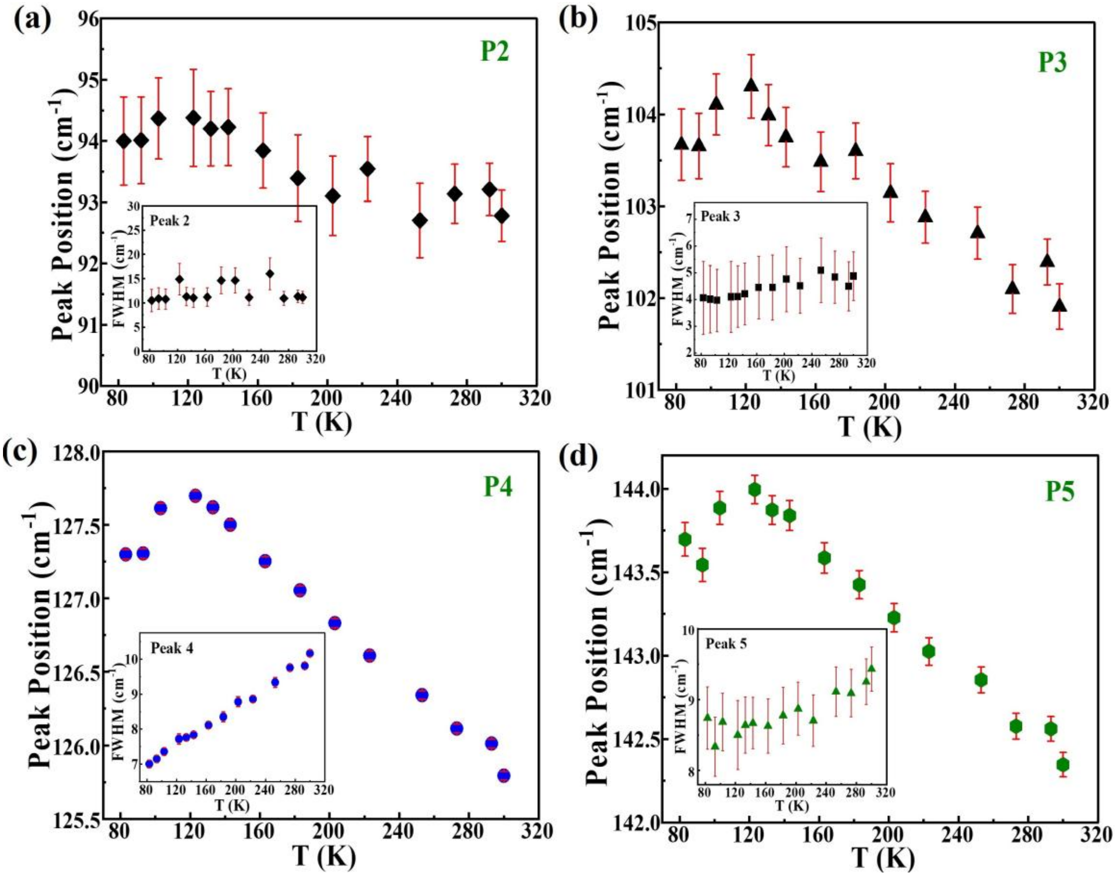


**Figure S18.** *(a-d) The temperature dependence of the phonon frequencies (peak positions), for the four Raman modes (P2-P5). Inset: The temperature-dependent phonon linewidths for the corresponding modes.*

The phonon frequencies (peak positions), linewidths (FWHM), and intensity (the area under the curve) determined from the fitting process are plotted against temperature in Figures S18 and S19.

From the temperature-dependent peak positions data, significant deviations in phonon frequencies from the expected behavior are observed at temperatures below 110 K (~$T_{SR}$) for all four peaks, P2-P5, similar to the R190 data (Figure S12). As the temperature decreases towards $T_{SR}$, the peak positions exhibit a continuous blue shift. However, just below $T_{SR}$, an anomalous redshift extends down to our lowest measured temperature (~83 K). Careful observation indicates kink-like features near $T_C$. For peaks P2-P5, the FWHMs show a gradual decrease as the temperature decreases until $T_{SR}$. Near $T_{SR}$ and $T_C$, a clear kink is observed in the FWHMs.

Thus, the pronounced softening and broadening of phonons above $T_{SR}$ indicate significant anharmonicity. Additionally, the anomalous phonon hardening observed as the temperature increases until $T_{SR}$ can be attributed to enhanced spin-phonon coupling within this temperature range. Therefore, the interplay between strong spin-phonon coupling and intrinsic anharmonicity near $T_{SR}$ manifests as a change in slope behavior observed in the temperature-dependent phonon frequency data (Figure S18). This distinctive signature provides clear evidence of the spin reorientation transition, $T_{SR}$, in the $Fe_4GeTe_2$ system.

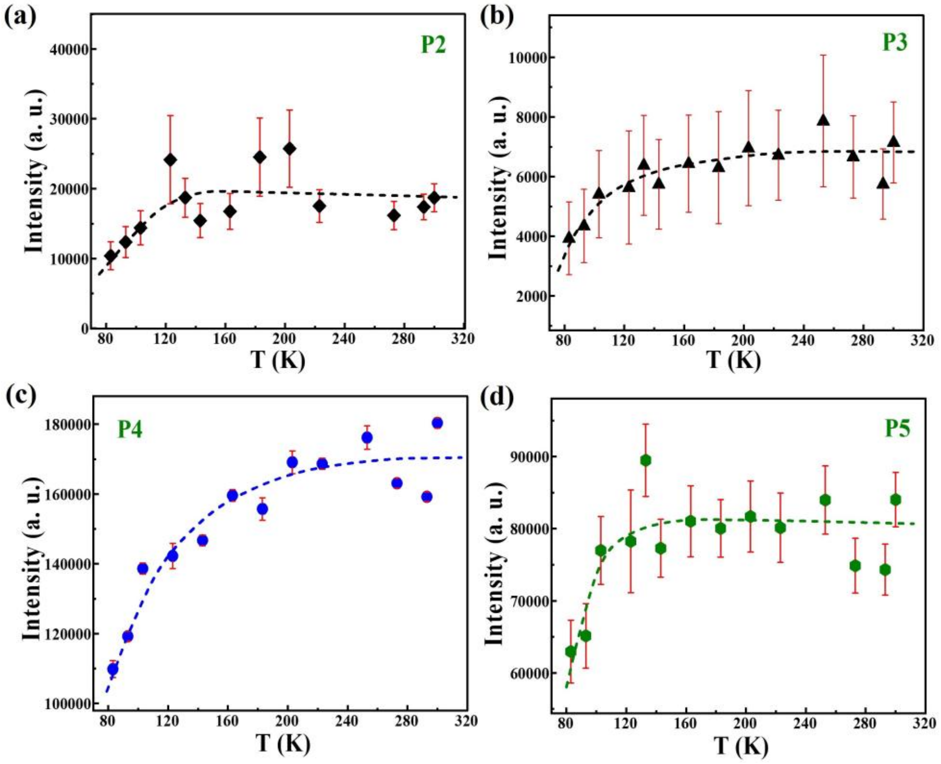


**Figure S19.** *(a-d) The temperature dependence of the intensity (area under the curve) for the four Raman modes (P2-P5). The dotted lines are the guide to the eye.*

**Section S8. Temperature dependent Raman measurement on 8 layered thin flake (R8) of $Fe_4GeTe_2$**

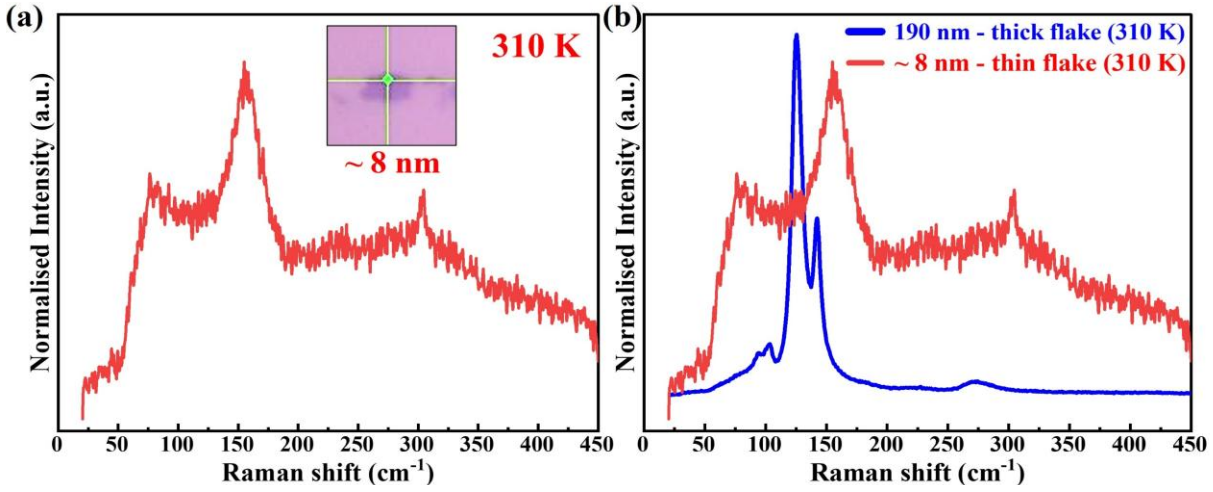


**Figure S20.** *(a) Raman spectra of 8 nm thin flake of $Fe_4GeTe_2$ at 310 K. (b) Comparison of this Raman spectra with R190 flake at same temperature.*

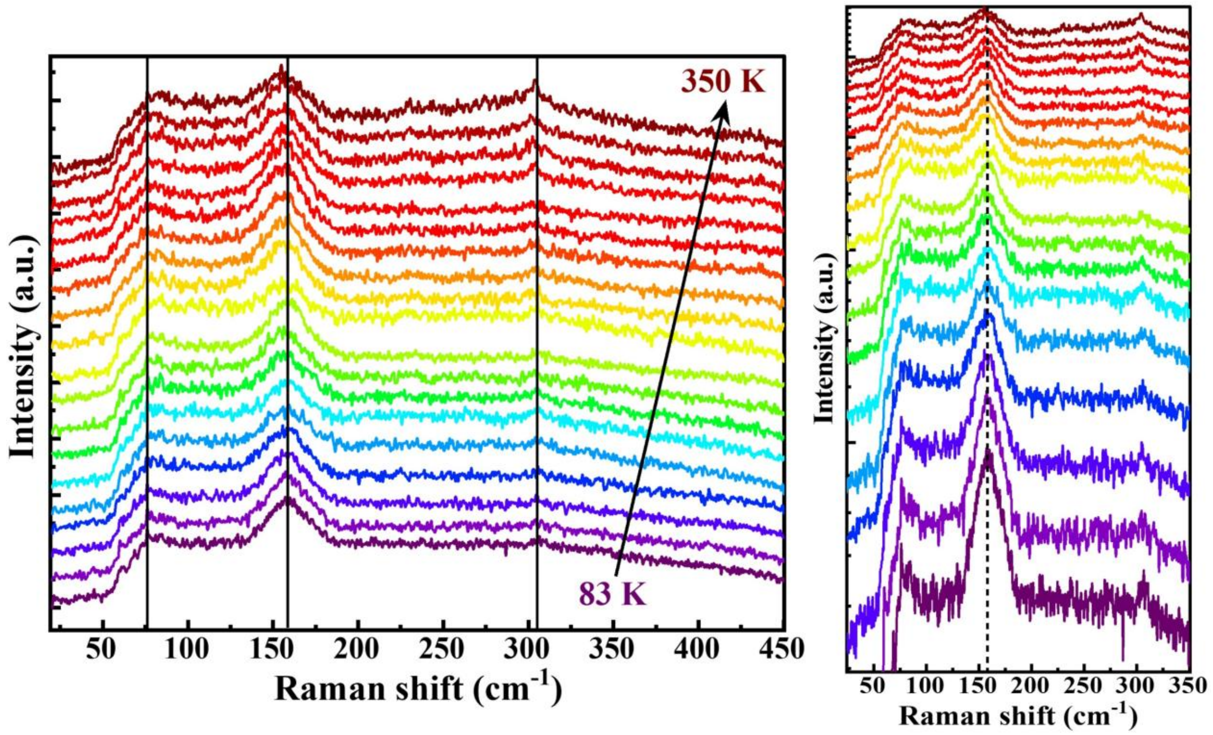


**Figure S21.** *(a) Temperature dependent Raman spectra of the 8 nm thin flake, showing no significant changes with temperature. (b) Temperature dependent Raman spectra plotted in semi-logarithmic scale, to visualise the changes.*

## Section S9. Raman measurements on other thin $Fe_4GeTe_2$ flakes

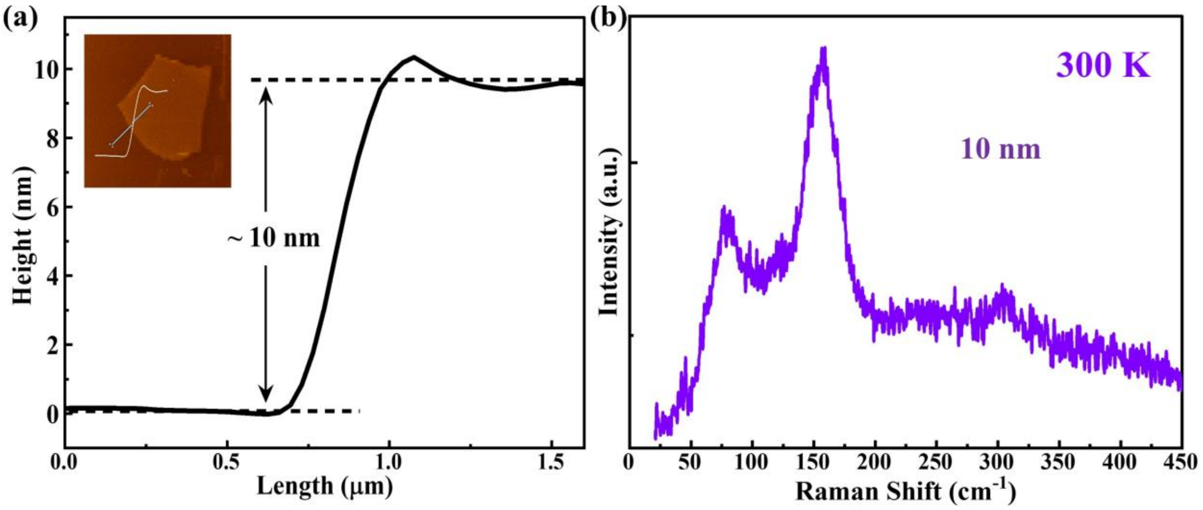


**Figure S22.** *(a) AFM image and the height profile of a thin flake (R10) of* $Fe_4GeTe_2$*. (b) Raman spectra of the R10 flake at 300 K.*

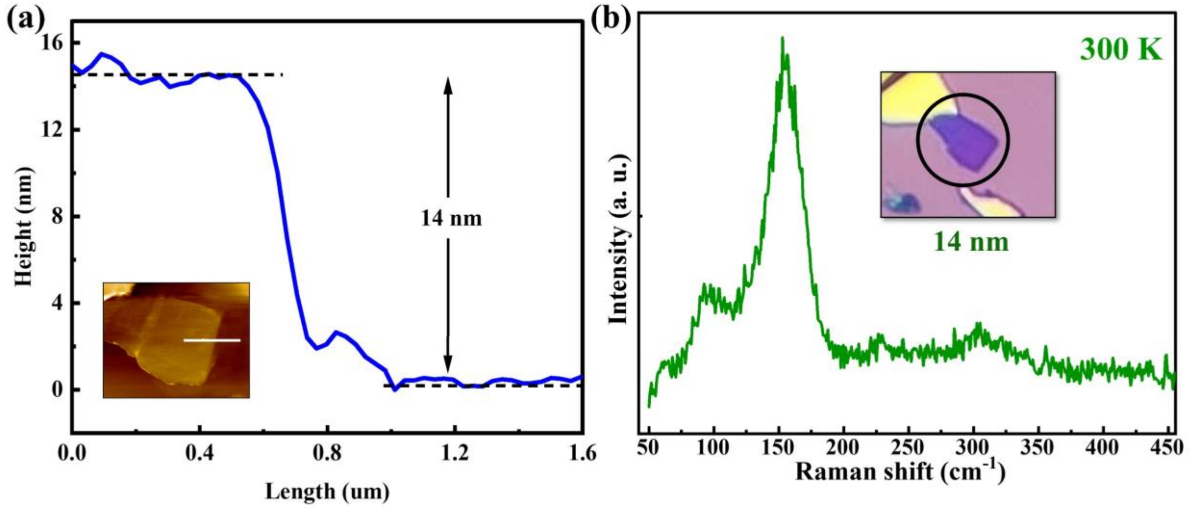


**Figure S23.** *(a) AFM image and the height profile of another thin flake (R14) of* $Fe_4GeTe_2$*. (b) Raman spectra of the 14 nm thin flake at 300 K.*

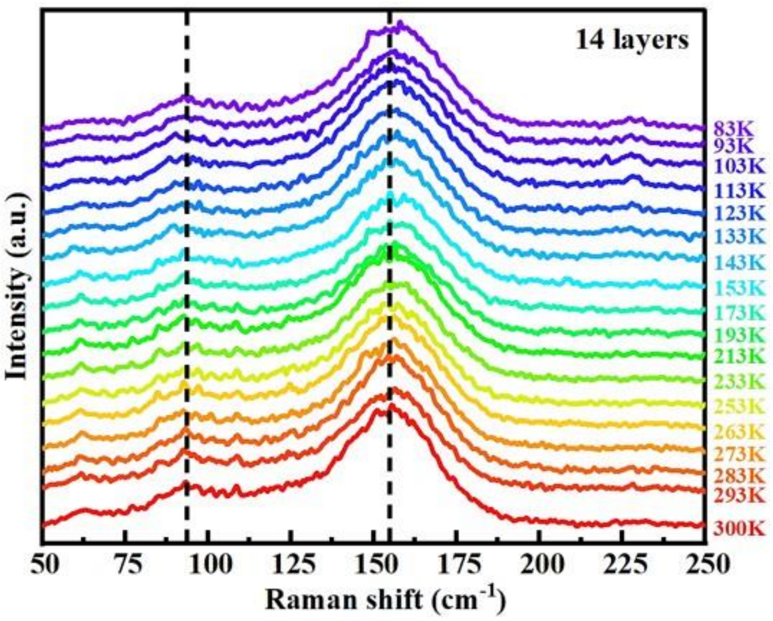


**Figure S24.** *(a) Temperature dependent Raman spectra of the 14 nm thin flake (R14), showing no observable changes of peak positions at temperatures below $T_{SR}$.*

**Section S10. Theoretical calculations**

- **Computational details**

Phonon dispersion curves at various temperatures were computed using VASP-Phonopy with GGA-PBE exchange-correlation functionals and van der Waals corrections[22–24]. XRD-derived temperature-dependent lattice parameters[3] were used to build initial $Fe_4GeTe_2$ structures. A 2×2×1 supercell was generated using the finite displacement method with atomic displacements of 0.0003 Å, yielding seven symmetrically distinct supercells.

Force constants for each symmetrically distinct supercell were calculated using first-principles VASP[22] computations. These constants, representing the interatomic potential, were subsequently processed with the Phonopy[23] code to construct the dynamical matrix. Diagonalization of this matrix results in the phonon frequencies, enabling the calculation of phonon dispersion curves along the high-symmetry path of the Brillouin zone. The dynamical matrices were computed over a q-point grid of 5×5×3. The plane-wave cutoff energy was set to 500 eV, with a Hellmann-Feynman force minimization criterion of 0.001 eV/Å and an electronic energy convergence threshold of $10^{-8}$ eV.

- **Phonon dispersion data**

To obtain a more comprehensive understanding of the lattice dynamics across different phonon modes, we have carried out a systematic theoretical investigation of the phonon dispersions and the corresponding vibrational behavior of $Fe_4GeTe_2$ across a temperature range from 10–320 K. The phonon dispersion data, as presented in Figure 1(e) (main text) and Supplementary Figure S25, are calculated along the high-symmetry path Γ–M–K–Γ of the Brillouin zone. To compare with the experimental data, we concentrated on the phonon modes at the zone center

(Γ-point) and the closest theoretical value to the experimental Raman-active modes at 300 K are presented in Table 1 (main text). The theoretically calculated phonon frequencies of 57.34 $cm^{-1}$, 78.13 $cm^{-1}$, 78.48 $cm^{-1}$, 119.3 $cm^{-1}$, 120.55 $cm^{-1}$, 148.71 $cm^{-1}$, 150.48 $cm^{-1}$, 183.3 $cm^{-1}$, 218.3 $cm^{-1}$, 280.74 $cm^{-1}$, and 286.3 $cm^{-1}$ resemble the experimental peaks P0, P1, P2, P3, P4, P5, P6, P7, P8, P9 and P10 respectively (see S26 and Fig. 1(f) in the main text). Such a resemblance indicates that the computational model effectively captures the fundamental vibrational dynamics of $Fe_4GeTe_2$.

**Table T5**: **Spin and orbital magnetic moments of Fe1 and Fe2 for different temperature-dependent crystal structures of $Fe_4GeTe_2$.**

| Temperature (K) | Moment for Fe1 ($\mu_B$) | | Moment for Fe2 ($\mu_B$) | |
|---|---|---|---|---|
| | Spin | Orbital | Spin | Orbital |
| 10 | 3.05 | 0.55 | 2.66 | 0.37 |
| 80 | 2.00 | 0.02 | 1.28 | 0.03 |

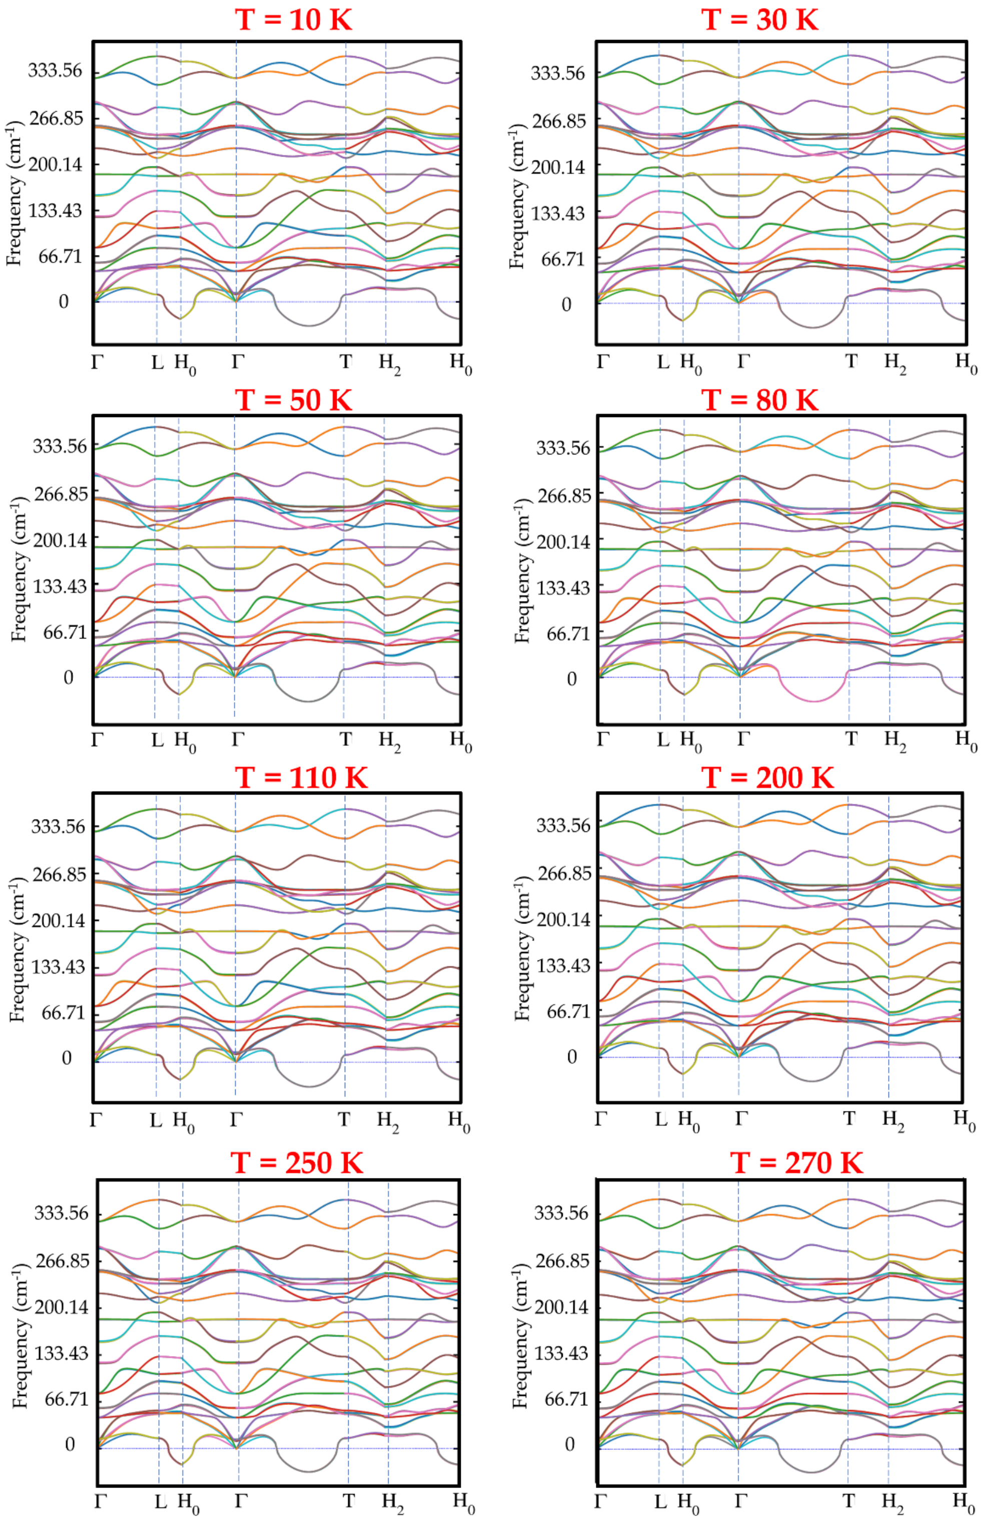


**Figure S25:** *Temperature dependent phonon dispersion plot for $Fe_4GeTe_2$, calculated using Phonopy-VASP. It shows the frequency dispersion of phonon modes across the Brillouin zone.*

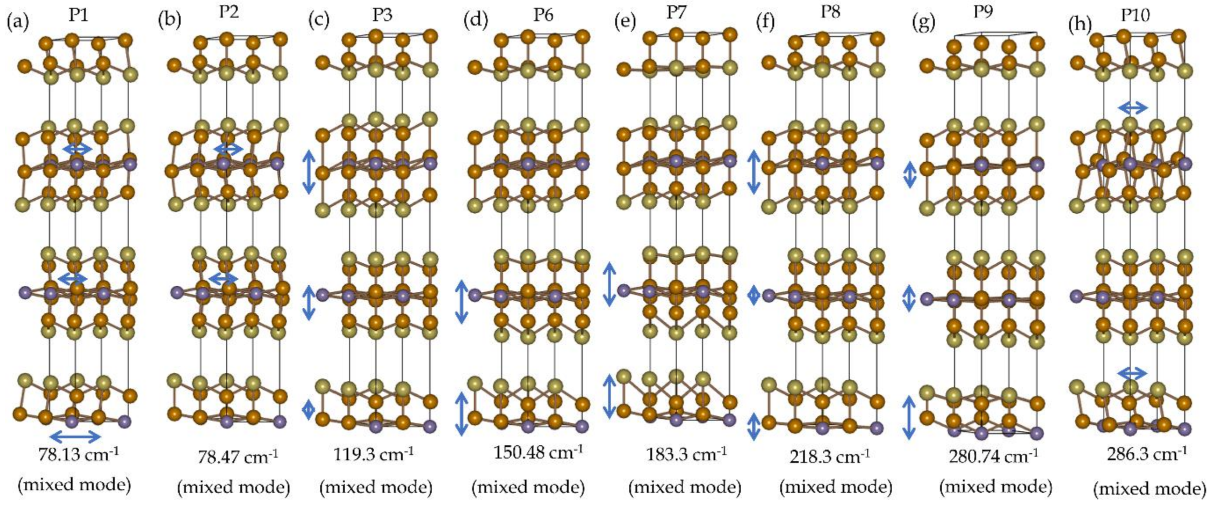


**Figure S26:** *Phonon mode frequencies and the associated vibrational patterns of $Fe_4GeTe_2$ calculated at a temperature of 300 K using Phonopy-VASP. The calculations highlight mode-specific behavior, providing insight into the phonon dispersion and symmetry characteristics.*

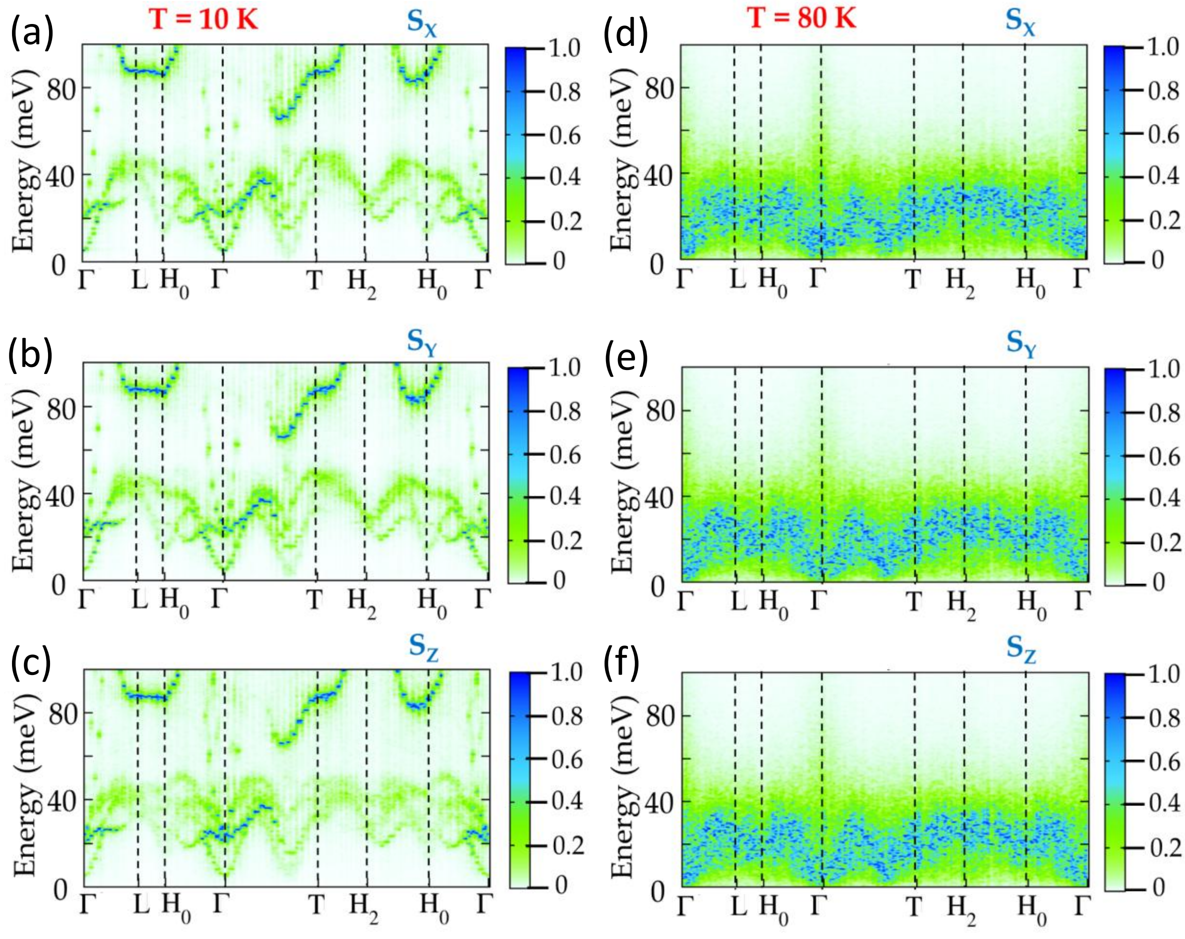


**Figure S27:** *Spin projected dynamical structure factors S(q,w) plotted along the high-symmetry paths for $Fe_4GeTe_2$ at T = 10 K (a, b, c) and T= 80 K (d, e, f).*

## References:


1. Mondal, S., Khan, N., Mishra, S. M., Satpati, B. & Mandal, P. Critical behavior in the van der Waals itinerant ferromagnet $Fe_4GeTe_2$. *Phys. Rev. B* **104**, 94405 (2021).

2. Pal, R. *et al.* Spin-reorientation driven emergent phases and unconventional magnetotransport in quasi-2D vdW ferromagnet $Fe_4GeTe_2$. *npj 2D Mater. Appl.* **8**, (2024).

3. Pal, R. *et al.* Disentangling the Unusual Magnetic Anisotropy of the Near-Room-Temperature Ferromagnet $Fe_4GeTe_2$. *Adv. Funct. Mater.* **34**, 2402551 (2024).

4. Seo, J. *et al.* Nearly room temperature ferromagnetism in a magnetic metal-rich van der Waals metal. *Sci. Adv.* **6**, 1–10 (2020).

5. Loudon, R. The Raman effect in crystals. *Adv. Phys.* **50**, 813–864 (2001).

6. Ferrari, A. C. *et al.* Raman spectrum of graphene and graphene layers. *Phys. Rev. Lett.* **97**, 1–4 (2006).

7. Ni, Z., Wang, Y., Yu, T. & Shen, Z. Raman spectroscopy and imaging of graphene. *Nano Res.* **1**, 273–291 (2008).

8. Graf, D., Molitor, F. & Ensslin, K. Spatially resolved Raman spectroscopy on single- and few-layer graphene Phonon spectrum of graphite. *Solid State Commun.*

9. Weerahennedige, H. *et al.* The effects of thickness, polarization, and strain on vibrational modes of 2D $Fe_3GeTe_2$. *Surfaces and Interfaces* **51**, 104797 (2024).

10. Lee, C. *et al.* Anomalous Lattice Vibrations of Single- and Few-Layer $MoS_2$. *ACS Nano* **4**, 2695–2700 (2010).

11. Bing, D. *et al.* Optical contrast for identifying the thickness of two-dimensional materials. *Opt. Commun.* **406**, 128–138 (2018).

12. Late, D. J., Liu, B., Matte, H. S. S. R., Rao, C. N. R. & Dravid, V. P. Rapid Characterization of Ultrathin Layers of Chalcogenides on $SiO_2$/Si Substrates. *Adv. Funct. Mater.* **22**, 1894–1905 (2012).

13. Gao, L., Ren, W., Li, F. & Cheng, H.-M. Total Color Difference for Rapid and Accurate Identification of Graphene. *ACS Nano* **2**, 1625–1633 (2008).

14. Ni, Z. H. *et al.* Graphene thickness determination using reflection and contrast spectroscopy. *Nano Lett.* **7**, 2758–2763 (2007).

15. Yang, H., Hu, H., Wang, Y. & Yu, T. Rapid and non-destructive identification of graphene oxide thickness using white light contrast spectroscopy. *Carbon N. Y.* **52**, 528–534 (2013).

16. Du, L. *et al.* Lattice Dynamics, Phonon Chirality, and Spin–Phonon Coupling in 2D Itinerant Ferromagnet $Fe_3GeTe_2$. *Adv. Funct. Mater.* **29**, 1–8 (2019).

17. Gong, C. *et al.* Discovery of intrinsic ferromagnetism in two-dimensional van der Waals crystals. *Nature* **546**, 265–269 (2017).

18. Huang, B. *et al.* Layer-dependent ferromagnetism in a van der Waals crystal down to the monolayer limit. *Nature* **546**, 270–273 (2017).

19. Shcherbakov, D. *et al.* Raman Spectroscopy, Photocatalytic Degradation, and Stabilization of Atomically Thin Chromium Tri-iodide. *Nano Lett.* **18**, 4214–4219 (2018).

20. Casto, L. D. *et al.* Strong spin-lattice coupling in $CrSiTe_3$. *APL Mater.* **3**, (2015).

21. Iturriaga, H. *et al.* Magnetic properties of intercalated quasi-2D $Fe_{3-x}GeTe_2$ van der Waals magnet. *npj 2D Mater. Appl.* **7**, 56 (2023).

22. Kresse, G. & Furthmüller, J. Efficiency of ab-initio total energy calculations for metals and semiconductors using a plane-wave basis set. *Comput. Mater. Sci.* **6**, 15–50 (1996).

23. Togo, A. & Tanaka, I. First principles phonon calculations in materials science. *Scr. Mater.* **108**, 1–5 (2015).

24. Perdew, J. P., Burke, K. & Ernzerhof, M. Generalized gradient approximation made simple. *Phys. Rev. Lett.* **77**, 3865–3868 (1996).
